# Supplementary material for: Launching Adversarial Attacks against Network Intrusion Detection Systems for IoT
Source: arXiv:2104.12426 source file (2021-04-26)
Supplement: Supplementary file 1 [file Appendix_C.tex]

\chapter{Project Diaries}
\label{app:proj_diaries}

% Template
% \includepdf[pages=1, width=\textwidth, frame, pagecommand=\subsection{TOKEN}, offset=0 -1.3cm]{./diaries/myPDF.pdf}

% May 12
\includepdf[pages=1, width=\textwidth, frame, pagecommand=\section{May 12. Project Kick-Off}, offset=0 -1.3cm]{./diaries/Diary_5_12.pdf}

% May 19
\includepdf[pages=1, width=\textwidth, frame, pagecommand=\section{May 19. Email Discussions}, offset=0 -1.3cm]{./diaries/Diary_5_19.pdf}

% June 11
\includepdf[pages=1, width=\textwidth, frame, pagecommand=\section{June 11. Diary Entry}, offset=0 -1.3cm]{./diaries/Diary_6_11.pdf}

% June 26
\includepdf[pages=1, width=\textwidth, frame, pagecommand=\section{June 26. Personal Diary Entry}, offset=0 -1.3cm]{./diaries/Diary_6_26.pdf}

% July 20 
\includepdf[pages=1, width=\textwidth, frame, pagecommand=\section{July 20. Project Meeting}, offset=0 -1.3cm]{./diaries/Diary_7_20.pdf}

% July 27
\includepdf[pages=1, width=\textwidth, frame, pagecommand=\section{July 27. Project Meeting}, offset=0 -1.3cm]{./diaries/Diary_7_27.pdf}

% July 31
\includepdf[pages=1, width=\textwidth, frame, pagecommand=\section{July 31. Email Discussions}, offset=0 -1.3cm]{./diaries/Diary_7_31.pdf}

% August 5
\includepdf[pages=1, width=\textwidth, frame, pagecommand=\section{August 5. Personal Diary Entry}, offset=0 -1.3cm]{./diaries/Diary_8_5.pdf}

% August 10
\includepdf[pages=1, width=\textwidth, frame, pagecommand=\section{August 10. Email Discussions}, offset=0 -1.3cm]{./diaries/Diary_8_10.pdf}
