# Supplementary material for: Launching Adversarial Attacks against Network Intrusion Detection Systems for IoT
Source: arXiv:2104.12426 source file (2021-04-26)
Supplement: Supplementary file 2 [file ann_code.pdf]

# ANN Label Flip Activity

0. Import CleverHans/TensorFlow
1. Import the dataset
2. Prepare functions
3. Pre-process the data
4. Create and fit our ANN estimator
5. Prepare perturbing
6. Iteratively perturb more data
7. Plot the line graphs

## 0. Import CleverHans/Tensorflow

It is critical that we import the correct versions here

```
# Install bleeding edge version of cleverhans
!pip install
git+https://github.com/tensorflow/cleverhans.git#egg=cleverhans
import cleverhans
```

```
from tensorflow.keras.layers import Dropout, Dense
from cleverhans.future.tf2.attacks import fast_gradient_method
import tensorflow as tf
```

## 1. Import the dataset

```
import pandas as pd

training = pd.read_csv('/content/drive/My Drive/Bot-
IoT/UNSW_2018_IoT_Botnet_Final_10_best_Training.csv',
                       low_memory=False)
testing = pd.read_csv('/content/drive/My Drive/Bot-
IoT/UNSW_2018_IoT_Botnet_Final_10_best_Testing.csv',
                      low_memory=False)
```

## 2. Prepare functions

- MinMaxScaler
- OneHotEncoder
- `Recall`/`Precision`/`F1` calculators
- Plot confusion matrix

```
# Create MinMaxScaler function MMScaler
from sklearn.preprocessing import MinMaxScaler
import numpy as np

def MMScaler(data):
    """Funcion that will MinMaxScale the input dataframe"""
    scaler = MinMaxScaler()
    data_scaled = np.array(scaler.fit_transform(data))

    return data_scaled
```

```
# Create OneHotEncoder function
from sklearn.preprocessing import OneHotEncoder

def OHEncoder(data):
    oneHot = OneHotEncoder()
    OHEncoded = oneHot.fit_transform(data).toarray()

    return OHEncoded
```

```
# Calculate recall/ precision/ F1- scores manually
# because they are not the Keras model by default.
from keras import backend as K

def recall_m(y_true, y_pred):
    true_positives = K.sum(K.round(K.clip(y_true * y_pred, 0, 1)))
    possible_positives = K.sum(K.round(K.clip(y_true, 0, 1)))
    recall = true_positives / (possible_positives + K.epsilon())
    return recall

def precision_m(y_true, y_pred):
    true_positives = K.sum(K.round(K.clip(y_true * y_pred, 0, 1)))
    predicted_positives = K.sum(K.round(K.clip(y_pred, 0, 1)))
    precision = true_positives / (predicted_positives + K.epsilon())
    return precision

def f1_m(y_true, y_pred):
    precision = precision_m(y_true, y_pred)
    recall = recall_m(y_true, y_pred)
    return 2*((precision*recall)/(precision+recall+K.epsilon()))
```

```
def plot_conf_mat(cm, names, epsilon, targeted):
    """

    """
    fig, ax = plt.subplots(figsize = (4, 4))
```

```
    ax = sns.heatmap(cm,
                     annot=True,
                     cbar=False,
                     cmap=sns.light_palette((210, 90, 60), input="husl"),
                     fmt='d')

    ax.set_xticklabels(names)
    ax.set_yticklabels(names)
    if targeted == 'True':
        the_title = 'Targeted'
    if targeted == 'False':
        the_title = 'Non Targeted'
    ax.set(title=the_title+'_'+epsilon,
           xlabel="Predicted label",
           ylabel="True label")
    fig.savefig(fname='/content/drive/My Drive/Bot-
IoT/conf_mats/binary_'+targeted+'_'+epsilon+'.png', bbox_inches = "tight")
    fig.show();
```

## 3. Pre-process the data

```
drop_features = ['pkSeqID', 'proto',
                 'saddr', 'sport', 'daddr', 'dport',
                 'attack', 'category', 'subcategory']

X_train = training.drop(drop_features, axis=1)
X_test = testing.drop(drop_features, axis=1)

X_train_scaled = MMScaler(X_train)
X_test_scaled = MMScaler(X_test)
```

```
# Binary y
y_binary = training.iloc[:, -3:-2].values
yt_binary = testing.iloc[:, -3:-2].values

y_binary_train = OHEncoder(y_binary)
y_binary_test = OHEncoder(yt_binary)
```

```
y_multi = training.iloc[:, -2:-1].values
yt_multi = testing.iloc[:, -2:-1].values

y_multi_train = OHEncoder(y_multi)
y_multi_test = OHEncoder(yt_multi)
```

## 4. Create and fit our ANN estimator

```
binary_model = tf.keras.Sequential()
binary_model.add(Dense(20, input_dim=X_train_scaled.shape[1],
activation='tanh'))
binary_model.add(Dense(60, activation='tanh'))
binary_model.add(Dense(80, activation='tanh'))
binary_model.add(Dense(90, activation='tanh'))
binary_model.add(Dense(y_binary_train.shape[1], activation='sigmoid'))
binary_model.summary()

binary_model.compile(loss='categorical_crossentropy',
              optimizer='adam',
              metrics=['accuracy',f1_m,precision_m, recall_m])
```

```
multi_model = tf.keras.Sequential()
multi_model.add(Dense(20, input_dim=X_train_scaled.shape[1],
activation='tanh'))
multi_model.add(Dense(60, activation='tanh'))
multi_model.add(Dense(80, activation='tanh'))
multi_model.add(Dense(90, activation='tanh'))
multi_model.add(Dense(y_multi_train.shape[1], activation='sigmoid'))
multi_model.summary()

multi_model.compile(loss='categorical_crossentropy',
              optimizer='adam',
              metrics=['accuracy',f1_m,precision_m, recall_m])
```

```
from sklearn.utils.class_weight import compute_class_weight

y_binary_integers = np.argmax(y_binary_train, axis=1)
bin_class_weights = compute_class_weight('balanced',
np.unique(y_binary_integers), y_binary_integers)
d_bin_class_weight = dict(enumerate(bin_class_weights))

y_multi_integers = np.argmax(y_multi_train, axis=1)
multi_class_weights = compute_class_weight('balanced',
np.unique(y_multi_integers), y_multi_integers)
d_multi_class_weight = dict(enumerate(multi_class_weights))
```

```
binary_model.fit(X_train_scaled, y_multi_train,
                 epochs=4, batch_size=100,
                 class_weight=d_bin_class_weight)
```

```
binary_model.fit(X_train, y_multi_train,
                 epochs=4, batch_size=100,
                 class_weight=d_multi_class_weight)
```

```
bin_loss, bin_accuracy, bin_f1_score, bin_precision, bin_recall =
binary_model.evaluate(X_test_scaled, y_test,

batch_size=100)

print('    Test accuracy: ', round(bin_accuracy*100, 3))
print('    Test Loss     :', round(bin_loss*100, 3))
print('    Test recall:    ', round(bin_recall*100, 3))
print('    Test precision:', round(bin_precision*100, 3))
print('    Test F1_score: ', round(bin_f1_score*100, 3))
```

```
multi_loss, multi_accuracy, multi_f1_score, multi_precision, multi_recall =
binary_model.evaluate(X_test_scaled, y_test,

batch_size=100)

print('    Test accuracy: ', round(multi_accuracy*100, 3))
print('    Test Loss     :', round(multi_loss*100, 3))
print('    Test recall:    ', round(multi_recall*100, 3))
print('    Test precision:', round(multi_precision*100, 3))
print('    Test F1_score: ', round(multi_f1_score*100, 3))
```

## 5. Prepare perturbing

```
# Create logistic regression model
bin_logits_model =
tf.keras.Model(binary_model.input,binary_model.layers[-1].output)
multi_logits_model =
tf.keras.Model(multi_model.input,multi_model.layers[-1].output)
```

```
# Convert X_test to tensor
original_X_test = X_test_scaled
original_X_test =
tf.convert_to_tensor(original_X_test.reshape((len(X_test_scaled), 10)))
original_X_test # view it
```

## 6. Iteratively perturb more data

## Binary model

### Non targeted binary

```
# Non targeted
from sklearn.metrics import confusion_matrix
import numpy as np
import json

non_targeted_binary = {'accuracy':[],
                       'loss': [],
                       'recall': [],
                       'precision':[],
                       'f1':[]}

for i in range(0, 11):
    epsilon = i/10

    adversarial_bin_data_false = fast_gradient_method(bin_logits_model,
original_data,
                                                      epsilon, np.inf,
                                                      targeted=False)

    print(f"[+] Epsilon: {epsilon}")

    loss, accuracy, f1_score, precision, recall =
binary_model.evaluate(adversarial_bin_data_false,

y_test,

batch_size=100)
    print('    Test accuracy: ', round(accuracy, 3))
    print('    Test Loss     :', round(loss, 3))
    print('    Test recall:    ', round(recall, 3))
    print('    Test precision:', round(precision, 3))
    print('    Test F1_score: ', round(f1_score, 3))

    for key, value in non_targeted_binary.items():
        if key == 'accuracy':
            non_targeted_binary[key].append(accuracy)
        if key == 'loss':
            non_targeted_binary[key].append(loss)
        if key == 'recall':
            non_targeted_binary[key].append(recall)
        if key == 'precision':
            non_targeted_binary[key].append(precision)
        if key == 'f1':
            non_targeted_binary[key].append(f1_score)

    pred = np.argmax(binary_model.predict(adversarial_bin_data_false),
axis=1)
    y_binary_test_2 = np.argmax(y_binary, axis=1)
```

```
    cm = confusion_matrix(y_binary_test_2, pred)
    labels = ['Benign', 'Attack']
    np.set_printoptions(precision=2)
    plot_conf_mat(cm, names=labels, targeted="False", epsilon=str(epsilon))

print(non_targeted_binary)

with open("content/drive/My Drive/Bot-IoT/models/non_targeted_binary.json",
"w") as file:
    json.dump(non_targeted_binary, file)
```

**Targeted binary**

```
# Non targeted
from sklearn.metrics import confusion_matrix
import numpy as np
import json

targeted_binary = {'accuracy':[],
                   'loss': [],
                   'recall': [],
                   'precision':[],
                   'f1':[]}

for i in range(0, 11):
    epsilon = i/10

    adversarial_bin_data_true = fast_gradient_method(bin_logits_model,
original_data,
                                                     epsilon, np.inf,
                                                     targeted=True)

    print(f"[+] Epsilon: {epsilon}")

    loss, accuracy, f1_score, precision, recall =
binary_model.evaluate(adversarial_bin_data_true,

y_test,

batch_size=100)
    print('     Test accuracy: ', round(accuracy, 3))
    print('     Test Loss     :', round(loss, 3))
    print('     Test recall:    ', round(recall, 3))
    print('     Test precision:', round(precision, 3))
    print('     Test F1_score: ', round(f1_score, 3))

    for key, value in targeted_binary.items():
        if key == 'accuracy':
            targeted_binary[key].append(accuracy)
        if key == 'loss':
            targeted_binary[key].append(loss)
        if key == 'recall':
```

```
            targeted_binary[key].append(recall)
        if key == 'precision':
            targeted_binary[key].append(precision)
        if key == 'f1':
            targeted_binary[key].append(f1_score)

    pred = np.argmax(binary_model.predict(adversarial_bin_data_true),
axis=1)
    y_binary_test_3 = np.argmax(y_binary, axis=1)
    cm = confusion_matrix(y_binary_test_3, pred)
    labels = ['Benign', 'Attack']
    np.set_printoptions(precision=2)
    plot_conf_mat(cm, names=labels, targeted="True", epsilon=str(epsilon))

print(targeted_binary)

with open("content/drive/My Drive/Bot-IoT/models/targeted_binary.json",
"w") as file:
    json.dump(targeted_binary, file)
```

Multi-Classification

**Non targeted multi classification**

```
from sklearn.metrics import confusion_matrix
import numpy as np
import json

non_targeted_multi = {'accuracy':[],
                      'loss': [],
                      'recall': [],
                      'precision':[],
                      'f1':[]}

for i in range(0, 11):
    epsilon = 1/10
    adversarial_multi_data_false = fast_gradient_method(multi_logits_model,
                                                         original_data,
                                                         epsilon, np.inf,
                                                         targeted=False)

    loss, accuracy, f1_score, precision, recall =
multi_model.evaluate(adversarial_multi_data_false,

y_test,

batch_size=100)

    print('    Test accuracy: ', round(accuracy, 3))
    print('    Test Loss     :', round(loss, 3))
    print('    Test recall:    ', round(recall, 3))
```

```
    print('    Test precision:', round(precision, 3))
    print('    Test F1_score: ', round(f1_score, 3))

    for key, value in non_targeted_multi.items():
        if key == 'accuracy':
            non_targeted_multi[key].append(accuracy)
        if key == 'loss':
            non_targeted_multi[key].append(loss)
        if key == 'recall':
            non_targeted_multi[key].append(recall)
        if key == 'precision':
            non_targeted_multi[key].append(precision)
        if key == 'f1':
            non_targeted_multi[key].append(f1_score)

    pred = np.argmax(multi_model.predict(adversarial_multi_data_false),
axis=1)
    y_multi_test_2 = np.argmax(y_test, axis=1)
    cm = confusion_matrix(y_multi_test_2, pred)
    labels = ['DDoS', 'DoS', 'Benign', 'Reconnaissance', 'Theft']
    np.set_printoptions(precision=2)
    plot_conf_mat(cm, names=labels, targeted="False", epsilon=str(epsilon))

print(non_targeted_multi)

with open("content/drive/My Drive/Bot-IoT/models/non_targeted_multi.json",
"w") as file:
    json.dump(non_targeted_multi, file)
```

#### Targeted multi classification

```
from sklearn.metrics import confusion_matrix
import numpy as np
import json

targeted_multi = {'accuracy':[],
                      'loss': [],
                      'recall': [],
                      'precision':[],
                      'f1':[]}

for i in range(0, 11):
    epsilon = 1/10
    adversarial_multi_data_true = fast_gradient_method(multi_logits_model,
                                                       original_data,
                                                       epsilon, np.inf,
                                                       targeted=True)

    loss, accuracy, f1_score, precision, recall =
multi_model.evaluate(adversarial_multi_data_true,

y_test,
```

```
batch_size=100)

    print('    Test accuracy: ', round(accuracy, 3))
    print('    Test Loss     :', round(loss, 3))
    print('    Test recall:    ', round(recall, 3))
    print('    Test precision:', round(precision, 3))
    print('    Test F1_score: ', round(f1_score, 3))

    for key, value in targeted_multi.items():
        if key == 'accuracy':
            targeted_multi[key].append(accuracy)
        if key == 'loss':
            targeted_multi[key].append(loss)
        if key == 'recall':
            targeted_multi[key].append(recall)
        if key == 'precision':
            targeted_multi[key].append(precision)
        if key == 'f1':
            targeted_multi[key].append(f1_score)

    pred = np.argmax(multi_model.predict(adversarial_multi_data_true),
axis=1)
    y_multi_test_3 = np.argmax(y_test, axis=1)
    cm = confusion_matrix(y_multi_test_3, pred)
    labels = ['DDoS', 'DoS', 'Benign', 'Reconnaissance', 'Theft']
    np.set_printoptions(precision=2)
    plot_conf_mat(cm, names=labels, targeted="True", epsilon=str(epsilon))

print(targeted_multi)

with open("content/drive/My Drive/Bot-IoT/models/targeted_multi.json", "w")
as file:
    json.dump(targeted_multi, file)
```

## 7. Plot the line graphs

Binary graphs

```
import matplotlib.pyplot as plt
import seaborn as sns
import json

with open("content/drive/My Drive/Bot-IoT/models/non_targeted_binary.json",
"r") as file:
    non_targeted_binary = json.load(non_targeted_binary)

fig, axs = plt.subplots(3, 2, figsize=(8,6))
Xscale = [0, 0.1, 0.2, 0.3, 0.4, 0.5, 0.6, 0.7, 0.8, 0.9, 1.0]

axs[0, 0].plot(Xscale, non_targeted_binary['accuracy'], 'tab:red')
```

```
axs[0, 0].set_title('Accuracy Score')
axs[0, 0].set_ylim([0, 1.1])
axs[0, 1].plot(Xscale, non_targeted_binary['loss'], 'tab:green')
axs[0, 1].set_title('Loss Score')
axs[0, 1].set_ylim([0, 1.1])
axs[1, 0].plot(Xscale, non_targeted_binary['precision'], 'tab:orange')
axs[1, 0].set_title('Precision Score')
axs[1, 0].set_ylim([0, 1.1])
axs[1, 1].plot(Xscale, non_targeted_binary['f1'], 'tab:purple')
axs[1, 1].set_title('F1 Score')
axs[1, 1].set_ylim([0, 1.1])
axs[2, 0].plot(Xscale, non_targeted_binary['recall'])
axs[2, 0].set_title('Recall Score')
axs[2, 0].set_ylim([0, 1.1])
fig.delaxes(axs[2][1])

fig.tight_layout(pad=2)

for ax in axs.flat:
    ax.set(xlabel='Epsilon Value')

fig.show();
```

```
import matplotlib.pyplot as plt
import seaborn as sns
import json

with open("content/drive/My Drive/Bot-IoT/models/targeted_binary.json",
"r") as file:
    targeted_binary = json.load(targeted_binary)

fig, axs = plt.subplots(3, 2, figsize=(8,6))
Xscale = [0, 0.1, 0.2, 0.3, 0.4, 0.5, 0.6, 0.7, 0.8, 0.9, 1.0]

axs[0, 0].plot(Xscale, targeted_binary['accuracy'], 'tab:red')
axs[0, 0].set_title('Accuracy Score')
axs[0, 0].set_ylim([0, 1.1])
axs[0, 1].plot(Xscale, targeted_binary['loss'], 'tab:green')
axs[0, 1].set_title('Loss Score')
axs[0, 1].set_ylim([0, 1.1])
axs[1, 0].plot(Xscale, targeted_binary['precision'], 'tab:orange')
axs[1, 0].set_title('Precision Score')
axs[1, 0].set_ylim([0, 1.1])
axs[1, 1].plot(Xscale, targeted_binary['f1'], 'tab:purple')
axs[1, 1].set_title('F1 Score')
axs[1, 1].set_ylim([0, 1.1])
axs[2, 0].plot(Xscale, targeted_binary['recall'])
axs[2, 0].set_title('Recall Score')
axs[2, 0].set_ylim([0, 1.1])
fig.delaxes(axs[2][1])
```

```
fig.tight_layout(pad=2)

for ax in axs.flat:
    ax.set(xlabel='Epsilon Value')

fig.show();
```

```
# Focus on accuracy/recall score non-targeted
import matplotlib.pyplot as plt
import seaborn as sns
import json

acc_rec_bin_non_targeted = {'accuracy': non_targeted_binary['accuracy'],
                              'recall': non_targeted_binary['recall']}

Xscale = [0, 0.1, 0.2, 0.3, 0.4, 0.5, 0.6, 0.7, 0.8, 0.9, 1.0]

fig, axs = plt.subplots(1, 1, figsize=(7,5))

axs.plot(Xscale, acc_rec_bin_non_targeted['accuracy'], label='Accuracy')
axs.plot(Xscale, acc_rec_bin_non_targeted['recall'], '--', label='Recall')
axs.set_title('Comparing Accuracy vs. Recall score in Targeted Multi Class
Model')
axs.set_ylim([0.4, 1])

fig.tight_layout(pad=2)

axs.set_xlabel('Epsilon Value')
axs.set_ylabel('Recall Score')
axs.legend()
leg = ax.legend();
```

```
# Focus on accuracy/recall score targeted
import matplotlib.pyplot as plt
import seaborn as sns
import json

acc_rec_bin_targeted = {'accuracy': targeted_binary['accuracy'],
                        'recall': targeted_binary['recall']}

Xscale = [0, 0.1, 0.2, 0.3, 0.4, 0.5, 0.6, 0.7, 0.8, 0.9, 1.0]

fig, axs = plt.subplots(1, 1, figsize=(7,5))

axs.plot(Xscale, acc_rec_bin_targeted['accuracy'], label='Accuracy')
axs.plot(Xscale, acc_rec_bin_targeted['recall'], '--', label='Recall')
axs.set_title('Comparing Accuracy vs. Recall score in Targeted Multi Class
Model')
axs.set_ylim([0.4, 1])
```

```
fig.tight_layout(pad=2)

axs.set_xlabel('Epsilon Value')
axs.set_ylabel('Recall Score')
axs.legend()
leg = ax.legend();
```

Multi-classification graphs

```
import matplotlib.pyplot as plt
import seaborn as sns
import json

with open("content/drive/My Drive/Bot-IoT/models/non_targeted_multi.json",
"r") as file:
    non_targeted_multi = json.load(non_targeted_multi)

fig, axs = plt.subplots(3, 2, figsize=(8,6))
Xscale = [0, 0.1, 0.2, 0.3, 0.4, 0.5, 0.6, 0.7, 0.8, 0.9, 1.0]

axs[0, 0].plot(Xscale, non_targeted_multi['accuracy'], 'tab:red')
axs[0, 0].set_title('Accuracy Score')
axs[0, 0].set_ylim([0, 1])
axs[0, 1].plot(Xscale, non_targeted_multi['loss'], 'tab:green')
axs[0, 1].set_title('Loss Score')
axs[0, 1].set_ylim([0, 2])
axs[1, 0].plot(Xscale, non_targeted_multi['precision'], 'tab:orange')
axs[1, 0].set_title('Precision Score')
axs[1, 0].set_ylim([0, 1])
axs[1, 1].plot(Xscale, non_targeted_multi['f1'], 'tab:purple')
axs[1, 1].set_title('F1 Score')
axs[1, 1].set_ylim([0, 1])
axs[2, 0].plot(Xscale, non_targeted_multi['recall'])
axs[2, 0].set_title('Recall Score')
axs[2, 0].set_ylim([0, 1])
fig.delaxes(axs[2][1])

fig.tight_layout(pad=2)

for ax in axs.flat:
    ax.set(xlabel='Epsilon Value', ylabel='Score')
fig.show();
```

```
import matplotlib.pyplot as plt
import seaborn as sns
import json

with open("content/drive/My Drive/Bot-IoT/models/targeted_multi.json", "r")
```

```
as file:
    targeted_multi = json.load(targeted_multi)

fig, axs = plt.subplots(3, 2, figsize=(8,6))
Xscale = [0, 0.1, 0.2, 0.3, 0.4, 0.5, 0.6, 0.7, 0.8, 0.9, 1.0]

axs[0, 0].plot(Xscale, targeted_multi['accuracy'], 'tab:red')
axs[0, 0].set_title('Accuracy Score')
axs[0, 0].set_ylim([0, 1])
axs[0, 1].plot(Xscale, targeted_multi['loss'], 'tab:green')
axs[0, 1].set_title('Loss Score')
axs[0, 1].set_ylim([0, 2])
axs[1, 0].plot(Xscale, targeted_multi['precision'], 'tab:orange')
axs[1, 0].set_title('Precision Score')
axs[1, 0].set_ylim([0, 1])
axs[1, 1].plot(Xscale, targeted_multi['f1'], 'tab:purple')
axs[1, 1].set_title('F1 Score')
axs[1, 1].set_ylim([0, 1])
axs[2, 0].plot(Xscale, targeted_multi['recall'])
axs[2, 0].set_title('Recall Score')
axs[2, 0].set_ylim([0, 1])
fig.delaxes(axs[2][1])

fig.tight_layout(pad=2)

for ax in axs.flat:
    ax.set(xlabel='Epsilon Value', ylabel='Score')
fig.show();
```

```
# Focus on accuracy/recall score non-targeted
import matplotlib.pyplot as plt
import seaborn as sns
import json

acc_rec_multi_non_targeted = {'accuracy': non_targeted_multi['accuracy'],
                              'recall': non_targeted_multi['recall']}

Xscale = [0, 0.1, 0.2, 0.3, 0.4, 0.5, 0.6, 0.7, 0.8, 0.9, 1.0]

fig, axs = plt.subplots(1, 1, figsize=(7,5))

axs.plot(Xscale, acc_rec_multi_non_targeted['accuracy'], label='Accuracy')
axs.plot(Xscale, acc_rec_multi_non_targeted['recall'], '--',
label='Recall')
axs.set_title('Comparing Accuracy vs. Recall score in Targeted Multi Class
Model')
axs.set_ylim([0.4, 1])

fig.tight_layout(pad=2)

axs.set_xlabel('Epsilon Value')
```

```
axs.set_ylabel('Recall Score')
axs.legend()
leg = ax.legend();
```

```
# Focus on accuracy/recall score targeted
import matplotlib.pyplot as plt
import seaborn as sns
import json

acc_rec_multi_targeted = {'accuracy': targeted_multi['accuracy'],
                          'recall': targeted_multi['recall']}

Xscale = [0, 0.1, 0.2, 0.3, 0.4, 0.5, 0.6, 0.7, 0.8, 0.9, 1.0]

fig, axs = plt.subplots(1, 1, figsize=(7,5))

axs.plot(Xscale, acc_rec_multi_targeted['accuracy'], label='Accuracy')
axs.plot(Xscale, acc_rec_multi_targeted['recall'], '--', label='Recall')
axs.set_title('Comparing Accuracy vs. Recall score in Targeted Multi Class
Model')
axs.set_ylim([0.4, 1])

fig.tight_layout(pad=2)

axs.set_xlabel('Epsilon Value')
axs.set_ylabel('Recall Score')
axs.legend()
leg = ax.legend();
```
