# Supplementary material for: Launching Adversarial Attacks against Network Intrusion Detection Systems for IoT
Source: arXiv:2104.12426 source file (2021-04-26)

| ID | Task Name | Duration | Start | Finish |
|---|---|---|---|---|
| 1 | **Phase 1** | **20 days** | **Sun 10/05/20** | **Fri 05/06/20** |
| 2 | Contact supervisors | 6 days | Sun 10/05/20 | Fri 15/05/20 |
| 3 | Research Proposal | 15 days | Mon 18/05/20 | Fri 05/06/20 |
| 4 | **Initial Report** | **15 days** | **Sat 06/06/20** | **Fri 26/06/20** |
| 5 | Create project plan | 2 days | Sat 06/06/20 | Sun 07/06/20 |
| 6 | Literature Search | 7 days | Mon 08/06/20 | Tue 16/06/20 |
| 7 | Document literature search | 6 days | Wed 17/06/20 | Wed 24/06/20 |
| 8 | Finalise initial report | 3 days | Wed 24/06/20 | Fri 26/06/20 |
| 9 | Initial Report Handin | 0 days | Fri 26/06/20 | Fri 26/06/20 |
| 10 | **Methodology** | **7 days** | **Mon 29/06/20** | **Tue 07/07/20** |
| 11 | Requirements Analysis | 2 days | Mon 29/06/20 | Tue 30/06/20 |
| 12 | Evaluate Tools | 2 days | Wed 01/07/20 | Thu 02/07/20 |
| 13 | Document Methodology | 3 days | Fri 03/07/20 | Tue 07/07/20 |
| 14 | **Implementation** | **18 days** | **Wed 08/07/20** | **Fri 31/07/20** |
| 15 | Data modelling | 3 days | Wed 08/07/20 | Fri 10/07/20 |
| 16 | Data pre-processing | 4 days | Mon 13/07/20 | Thu 16/07/20 |
| 17 | Model Training and improvement | 8 days | Fri 17/07/20 | Tue 28/07/20 |
| 18 | Document Implementation | 3 days | Wed 29/07/20 | Fri 31/07/20 |
| 19 | **Results and Evaluation** | **7 days** | **Mon 03/08/20** | **Tue 11/08/20** |
| 20 | Scores comparison | 3 days | Mon 03/08/20 | Wed 05/08/20 |
| 21 | Evaluation of project | 4 days | Thu 06/08/20 | Tue 11/08/20 |

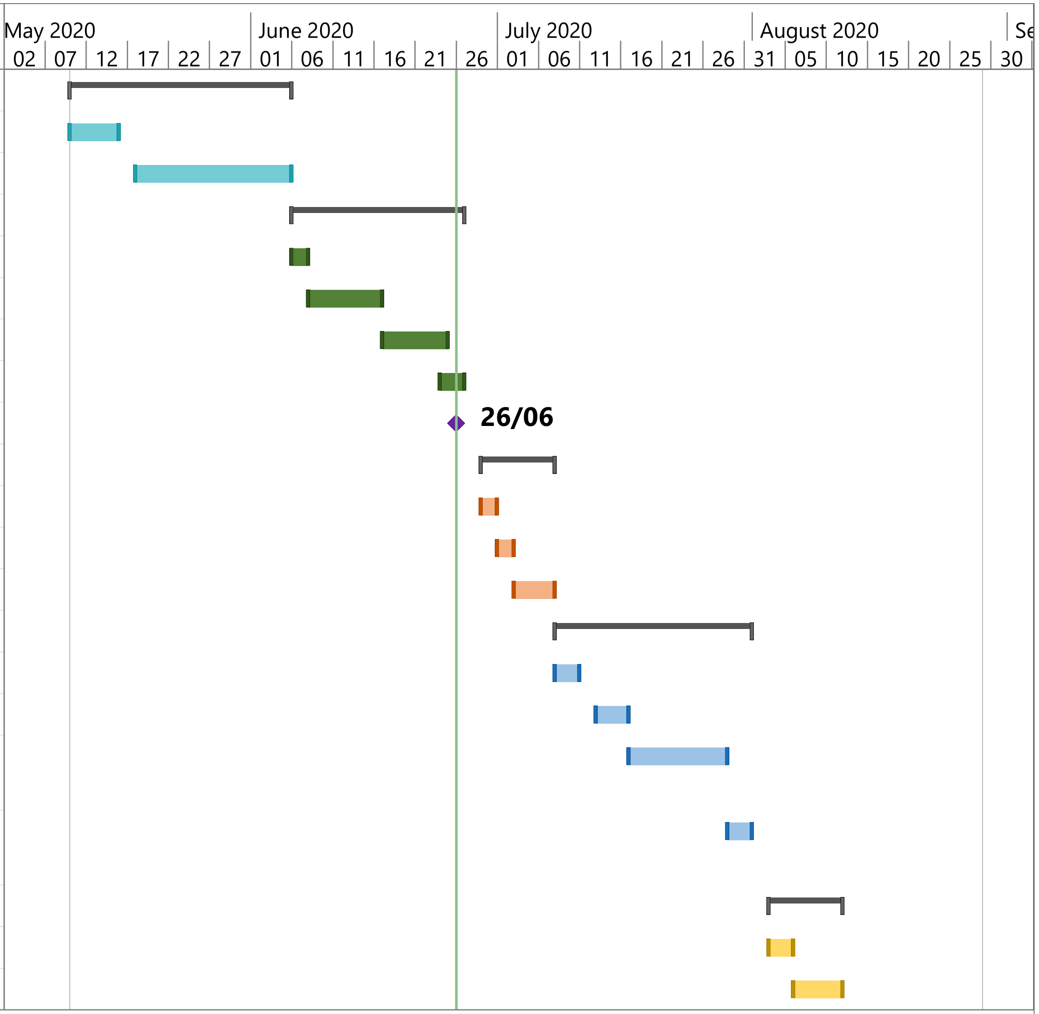


Project: Plan
Date: Fri 26/06/20

Task
Split
Milestone
Summary
Project Summary
Inactive Task
Inactive Milestone
Inactive Summary
Manual Task
Duration-only
Manual Summary Rollup
Manual Summary
Start-only
Finish-only
External Tasks
External Milestone
Deadline
Progress
Manual Progress

| ID | Task Name | Duration | Start | Finish |
|---|---|---|---|---|
| 22 | **Report Finalisation** | **4 days** | **Wed 12/08/20** | **Sun 16/08/20** |
| 23 | Write Abstract | 1 day | Wed 12/08/20 | Wed 12/08/20 |
| 24 | Document Introduction | 1 day | Thu 13/08/20 | Thu 13/08/20 |
| 25 | Polish report | 2 days | Fri 14/08/20 | Sun 16/08/20 |
| 26 | Dissertation Submission | 0 days | Mon 17/08/20 | Mon 17/08/20 |
| 27 | Viva held by | 0 days | Fri 28/08/20 | Fri 28/08/20 |

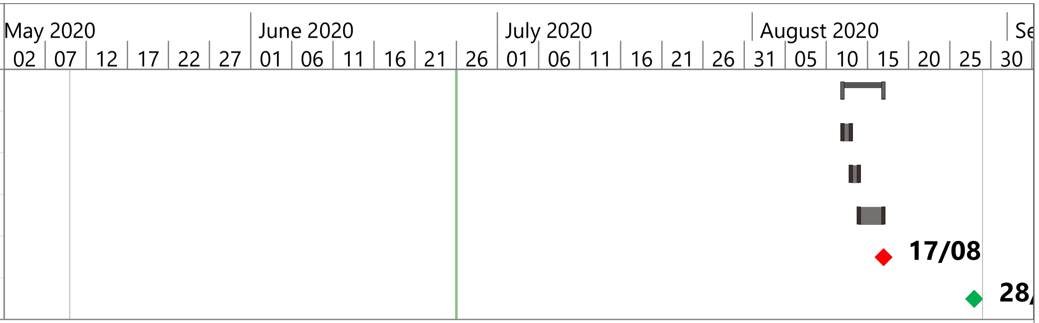


Project: Plan
Date: Fri 26/06/20

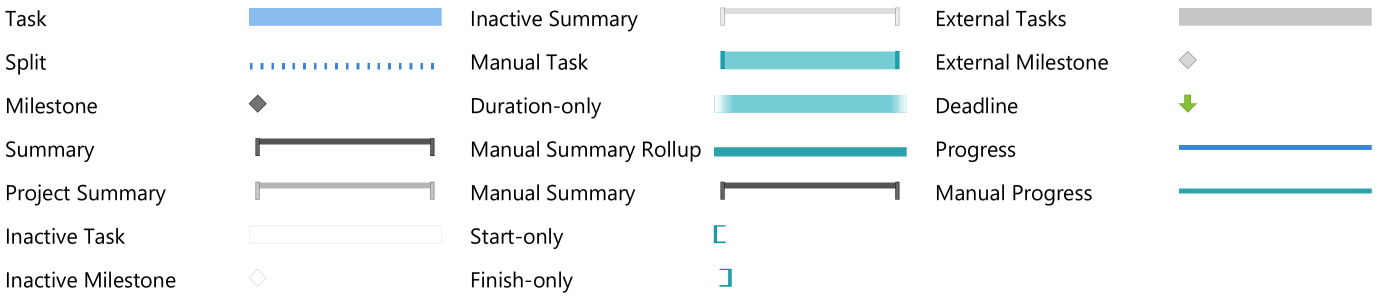

Supplement: Supplementary file 3 [file ganttChart.pdf]
