# Supplementary material for: Launching Adversarial Attacks against Network Intrusion Detection Systems for IoT
Source: arXiv:2104.12426 source file (2021-04-26)
Supplement: Supplementary file 4 [file proj_proposal.pdf]

EDINBURGH NAPIER UNIVERSITY SCHOOL OF COMPUTING

MSc RESEARCH PROPOSAL

The process of completing and reviewing the contents of this form is intended ensure that the proposed project is viable. It is also intended to increase the chances of a good pass. Much of the material produced while completing this form may be reused in the dissertation itself.

1. **Student details**

| | |
|---|---|
| First name | Oliver |
| Last (family) name | Thornewill von Essen |
| Edinburgh Napier matriculation number | 40210534 |

2. **Details of your programme of study**

| | |
|---|---|
| MSc Programme title | Advanced Security and Digital Forensics |
| Year that you started your diploma modules | 2019 |

3. **Project outline details**

Please suggest a title for your proposed project. If you have worked with a supervisor on this proposal, please provide the name. You are strongly advised to work with a member of staff when putting your proposal together.

| | |
|---|---|
| Title of the proposed project | Intrusion Detection using Machine Learning with a Bot-IoT dataset |
| Is your project appropriate to your programme of study? | Yes |
| Name of supervisor | Nikolaos Pitropakis |

4. **Brief description of the research area - background**

Please do not describe your project in this section. Instead, provide background information in the box below on the broad research area in which your project sits. You should write in narrative (not bullet points). The academic/theoretical basis of your description of the research area should be evident through the use of citations and references. Your description should be between half and one page in length.

Within an organization the network perimeter security must be maintained. The purpose of a secure network perimeter is to withhold the confidentiality, integrity, and availability (CIA) of an organization (Mukherjee & Todd, 1994). Both the annual cost and frequency of cyber-attacks are increasing (Sultana, Chilamkurti, Peng, & Alhadad, 2019). For this reason, the security staff within an organization will deploy a network intrusion system (NIDS) on different sensors within the network to detect adversarial traffic (Javaid, Niyaz, Sun, & Alam, 2016).

There are different types of NIDSs, ranging from deep packet inspection to packet header only examination. On the other hand, there are signature-based as well as anomaly-based intrusion detection systems. When considering deep packet inspection, there are analyses of the packet contents of a to identify malicious traffic. However, with end-to-end encryption services, deep packet inspection can often be thwarted and rendered ineffective (Sherry, Lan, Popa, & Ratnasamy, 2015). Packet inspection can be matched to find malicious traffic using two methods. Firstly, signature-based NIDS (SNIDS) which use predefined signatures to detect malicious traffic. SNIDS are good at detecting known attacks and report a low false-positive rate (FPR) which helps the security staff to save time when triaging events (Tang, Mhamdi, McLernon, Zaidi, & Ghogho, 2016). Secondly, there is anomaly-based NIDS (ANIDS) which compares traffic to a model of known good traffic and reports abnormal findings. ANIDS are useful when detecting unknown (zero-day) attacks; however, they often have the cost of a higher FPS compared to SNIDS FPR (Tang et al., 2016). Deployed NIDSs are often a hybrid combination of SNIDS and ANIDS.

Applying machine learning (ML) to NIDSs can be considered a different type of ANIDS, however ML applied to network security is a relatively new research area (Tang et al., 2016). ML is used to define rule sets which are useful to detect anomalous data. There are two primary types of ML. Firstly, there is supervised learning which entails using labelled data in training a model to predict unknown cases. (Mirsky, Doitshman, Elovici, & Shabtai, 2018). Secondly, there is unsupervised learning which does not use labelled data, but instead self identifies patterns in data to classify traffic as normal or anomalous (Mirsky et al., 2018). Research has demonstrated that ML can be more accurate at predicting normal or anomalous traffic as well as having a lower FPR when compared to non-ML based NIDS. (Gaikwad & Thool, 2015). A requirement of ML is a representative dataset which can be used to train and test the models. The KDD-CUP-1999 (Cup, 1999) dataset is commonly used in academic papers; however is criticized for being out of date as network practices have changed significantly. Therefore the trained models are no longer suitable for deployment (Tavallaee, Bagheri, Lu, & Ghorbani, 2009). As a solution, the NSL-KDD dataset (Tavallaee et al., 2009) was developed, which uses selective records from the KDD-CUP-1999 dataset. However, the NSL-KDD dataset still owns the problem that originating data is no longer applicable (Buczak & Guven, 2015).

IoT devices are growing in popularity in sectors such as medical, logistic tracking, smart cities, among other industries. The growth in demand inherently comes with a more significant number of attacks with new methods among the IoT devices as the attack surface for adversaries grows (Hodo et al., 2016). The Bot-IoT dataset has been released, which satisfies the requirement for a well-structured and representative data including simulated attacks (Koroniotis, Moustafa, Sitnikova, & Turnbull, 2019).

5. **Project outline for the work that you propose to complete**

Please complete the project outline in the box below. You should use the emboldened text as a framework. Your project outline should be between half and one page in length.

**The idea for this research arose from:**

When considering the modules which I enjoyed the most throughout the M.Sc. programme, I narrowed down that I wanted to carry out a project in either network security, insider threat, or malware analysis. I also knew that I wanted to undergo some machine learning activities as we had not covered it throughout the M.Sc. programme beyond some theory. Because malware analysis is my weakest of the three topics that I wanted to pursue, I discarded it. When considering insider threat and network security with each other, I thought that network security could potentially be a more profitable project for me in terms of career prospects. I approached Nick Pitropakis with some general ideas, and we narrowed down a specific topic which I will work on.

**The aims of the project are as follows:**

This project sets out to evaluate the dataset using different machine learning and deep learning (DL) models. The investigation will be completed by identifying the best features for the dataset, followed by hyperparameter analysis of the individual models.

**The main research questions that this work will address include:**

1. What are the current network intrusion system approaches and tools?
2. What is the threat landscape for IoT devices? What are the existing solutions to these risks?
3. What types of machine learning are there? Which of these will be most suitable for the selected dataset?
4. What are the most significant features of the dataset, and how can they be best selected to maintain or improve the accuracy?
5. How can ML or DL models be tuned to obtain better results?
6. How does the developed solution differ to what has been previously described?

**The software development/design work/other deliverable of the project will be:**

The exported Python machine learning models.

**The project deliverable will be evaluated as follows:**

Evaluation metrics such as the TPR/FPR, area under the receiver operating characteristic (ROC, AUC score), precision, recall, f1-score will be considered against the original metrics from the authors.

Continues on next page

**The project will involve the following research/field work/experimentation/evaluation:**

- Research:
    - Network intrusion detection systems, approaches, and existing tools
    - IoT security and their attack types
    - Types of machine learning and current approaches
    - Current mitigations to the IoT security risks
- Fieldwork/ Experimentation
    - Preparing the data for ML or DL models followed by an analysis of the data (e.g. correlation matrix or balanced data)
    - Train appropriate models, feature reduction, hyperparameter tuning
- Evaluation
    - Analysis of the results using the different models and comparison among them.
    - How the developed solution differs to previous knowledge, and why it is valuable.

**This work will require the use of specialist software:**
No specialist software is required beyond Python code.

**This work will require the use of specialist hardware:**
No specialist hardware is required.

**The project is being undertaken in collaboration with:**
Not applicable

6. **References**

Please supply details of all the material that you have referenced in sections 4 and 5 above. You should include at least three references, and these should be to high quality sources such as refereed journal and conference papers, standards or white papers. Please ensure that you use a standardised referencing style for the presentation of your references, e.g. APA, as outlined in the yellow booklet available from the School of Computing office and http://www.soc.napier.ac.uk/~cs104/mscdiss/moodlemirror/d2/2005_hall_referencing.pdf .


Buczak, A. L., & Guven, E. (2015). A survey of data mining and machine learning methods for cyber security intrusion detection. *IEEE Communications Surveys & Tutorials*, *18*(2), 1153–1176.

Gaikwad, D. P., & Thool, R. C. (2015). Intrusion detection system using bagging ensemble method of machine learning. In *2015 International Conference on Computing Communication Control and Automation* (pp. 291–295).

Hodo, E., Bellekens, X., Hamilton, A., Dubouilh, P.-L., Iorkyase, E., Tachtatzis, C., & Atkinson, R. (2016). Threat analysis of IoT networks using artificial neural network intrusion detection system. In *2016 International Symposium on Networks, Computers and Communications (ISNCC)* (pp. 1–6).

Javaid, A., Niyaz, Q., Sun, W., & Alam, M. (2016). A deep learning approach for network intrusion detection system. In *Proceedings of the 9th EAI International Conference on Bio-inspired Information and Communications Technologies (formerly BIONETICS)* (pp. 21–26).

Koroniotis, N., Moustafa, N., Sitnikova, E., & Turnbull, B. (2019). Towards the development of realistic botnet dataset in the internet of things for network forensic analytics: Bot-iot dataset. *Future Generation Computer Systems*, *100*, 779–796.

Mirsky, Y., Doitshman, T., Elovici, Y., & Shabtai, A. (2018). Kitsune: an ensemble of autoencoders for online network intrusion detection. *ArXiv Preprint ArXiv:1802.09089*.

Mukherjee, B., & Todd, L. (1994). Heberlein, and Karl N. Levitt. Network Intrusion Detection. *IEEE Network*, *8*(3), 26–41.

Sherry, J., Lan, C., Popa, R. A., & Ratnasamy, S. (2015). Blindbox: Deep packet inspection over encrypted traffic. In *Proceedings of the 2015 ACM Conference on Special Interest Group on Data Communication* (pp. 213–226).

Sultana, N., Chilamkurti, N., Peng, W., & Alhadad, R. (2019). Survey on SDN based network intrusion detection system using machine learning approaches. *Peer-to-Peer Networking and Applications*, *12*(2), 493–501.

Tang, T. A., Mhamdi, L., McLernon, D., Zaidi, S. A. R., & Ghogho, M. (2016). Deep learning approach for network intrusion detection in software defined networking. In *2016 International Conference on Wireless Networks and Mobile Communications (WINCOM)* (pp. 258–263).

Tavallaee, M., Bagheri, E., Lu, W., & Ghorbani, A. A. (2009). A detailed analysis of the KDD CUP 99 data set. In *2009 IEEE symposium on computational intelligence for security and defense applications* (pp. 1–6).

7. **Ethics**

If your research involves other people, privacy or controversial research there may be ethical issues to consider (please see the information on the module website). If the answer below is YES then you need to complete a research Ethics and Governance Approval form, available on the website: http://www.ethics.napier.ac.uk .

| | |
|---|---|
| Does this project have any ethical or governance issues related to working with, studying or observing other people? (YES/NO) | No |

8. **Confidentiality**

If your research is being done in conjunction with an outside firm or organisation, there may be issues of confidentiality or intellectual property.

| | |
|---|---|
| Does this project have any issues of confidentiality or intellectual property? (YES/NO) | No |

9. **Submitting your proposal**

1. Please save this file using your surname, e.g. macdonald_proposal.docx, and e-mail it to your supervisor, who will discuss it with you and suggest possible improvements.
2. When your supervisor is content with your proposal, submit it to the Research Proposal Upload link on Moodle, and email your internal examiner to notify them that you have submitted. They will leave feedback for you on Moodle.
3. Discuss your feedback from the internal examiner with your supervisor and if necessary make final changes to your proposal.
4. When you produce your dissertation, add your finalised proposal as an appendix.
