# Supplementary material for: Launching Adversarial Attacks against Network Intrusion Detection Systems for IoT
Source: arXiv:2104.12426 source file (2021-04-26)
Supplement: Supplementary file 5 [file svm_code.pdf]

# SVM Label Flip Activity

Stages:

1. Import the dataset
2. Prepare label flipping functions
3. Pre-process the data
4. Create the trusted SVM model
5. Perform the label flipping
6. Plot line graphs

## 1. Import the dataset

```
import pandas as pd

training = pd.read_csv("data/TrainTestSet/tenbest/tenbest-train-test-split/UNSW_2018_IoT_Botnet_Final_10_best_Training.csv")
testing = pd.read_csv("data/TrainTestSet/tenbest/tenbest-train-test-split/UNSW_2018_IoT_Botnet_Final_10_best_Testing.csv")
```

## 2. Prepare Functions

- MinMaxScaler
- Random Change
- Targeted Change
- Cross validation scorer
- Confusion Matrix
- ROC curve

```
# Create MinMaxScaler function MMScaler
from sklearn.preprocessing import MinMaxScaler
import numpy as np

def MMScaler(data):
    """Function that will MinMaxScale the input dataframe"""
    scaler = MinMaxScaler()
    data_scaled = np.array(scaler.fit_transform(data))

    return data_scaled
```

```
def randomChange(dataframe, n):
    """
    Function which selects a random sample of indexes
    from an input dataframe. The size of random samples
```

```
    is defined by the input n
    """
    change = dataframe.sample(int(n*len(dataframe))).index

    return change
```

```
import numpy as np

def targetChange(model, dataframe, n):
    """Inputs:
    Model: SVC model with decision_function
    dataframe: the features dataframe
    n: number of samples as a decimal percentage (5% = 0.05)
    """
    distances = model.decision_function(dataframe)
    abs_values = np.abs(distances)
    df = pd.DataFrame(data={'distance': distances,
                            'abs_value': abs_values},
                      columns=["distance", "abs_value"])

    change = df.sort_values(by=['abs_value']).head(int(len(df)*(n))).index

    return change
```

```
from sklearn.model_selection import cross_val_score

def show_scores(model, X, y):
    """
    Using X and y datasets, perform cross validation for
    accuracy, precision, recall and F1 scores
    """
    y_pred = model.predict(X)
    scores = {'accuracy': np.mean(cross_val_score(model, X, y, cv=4,
scoring='accuracy', n_jobs=-1)),
              'precision': np.mean(cross_val_score(model, X, y, cv=4,
scoring='precision', n_jobs=-1)),
              'recall': np.mean(cross_val_score(model, X, y, cv=4,
scoring='recall', n_jobs=-1)),
              'F1': np.mean(cross_val_score(model, X, y, cv=4,
scoring='f1', n_jobs=-1))}

    return scores
```

```
# Confusion Matrix
import matplotlib.pyplot as plt
import seaborn as sns
```

```
def plot_conf_mat(conf_mat, labels, flip, targeted):
    """
    plot conf mat w/ seaborn heatmap
    """
    fig, ax = plt.subplots(figsize=(4, 4))
    ax = sns.heatmap(conf_mat,
                     annot=True,
                     cbar=False,
                     cmap=sns.light_palette((210, 90, 60), input="husl"),
                     fmt="d")

    ax.set_xticklabels(labels)
    ax.set_yticklabels(labels)
    if targeted == 'True':
        the_title = 'Targeted'
    if targeted == 'False':
        the_title = 'Random Flip'
    ax.set(title=the_title+'_'+flip,
           xlabel="Predicted label",
           ylabel="True label")
    fig.savefig(fname='pictures/conf_mats/'+targeted+'_'+flip+'.png')
    fig.show()
```

```
# ROC Curve
import matplotlib.pyplot as plt
import seaborn as sns

def plot_roc_curve(fpr, tpr, auc, flip, targeted):
    """
    Plots ROC Curve
    """
    # plot roc
    plt.plot(fpr, tpr, label=f"ROC Curve (area = {auc:.3f})")
    plt.xlabel("False positive rate (FPR)")
    plt.ylabel("True positive rate (TPR)")
    plt.title("Receiver Operating Characteristic (ROC) Curve")
    plt.legend()
    plt.savefig(fname="pictures/roc_curves/"+targeted+flip+".png")
    plt.show()
```

## 3. Pre-process the data

```
# Define X_train and X_test

X_train = training.drop(['pkSeqID', 'proto',
                         'saddr', 'sport', 'daddr', 'dport',
                         'attack', 'category', 'subcategory'],
                        axis=1)
X_test = testing.drop(['pkSeqID', 'proto',
```

```
                              'saddr', 'sport', 'daddr', 'dport',
                              'attack', 'category', 'subcategory'],
                             axis=1)
```

```
import pandas as pd
# Scale the training/testing dataframe and create classification feature
X_train_scaled = MMScaler(X_train)
X_test_scaled = MMScaler(X_test)

y_train = training['attack'] # binary classification
y_test = testing['attack']   # binary classification

fullX_scaled = pd.concat([X_train_scaled, X_test_scaled])
fullY = pd.concat([y_train, y_test])
```

## 4. Create the trusted SVM model

```
from sklearn.svm import SVC

hyperparams = {'C'=1,
               'class_weight'='balanced',
               'kernel'='linear',
               'max_iter'=1000}

svcModel = SVC(**hyperparams)
svcModel.fit(X_train_scaled, y_train)
```

```
# Save model
import pickle
filename = 'models/SVM/trusted_model.pk1'
pickle.dump(svcModel, open(filename, 'wb'))
```

```
scores = show_scores(svcModel, fullX_scaled, fullY)

for scoring, score in scores.items():
    print(f"The {scoring} score: \t{(score)*100:.3f}%")
```

## 5. Perform Label Flipping

- Random SVC label flipping
- Targeted SVC label flipping

## Random SVC label flipping

Here we flip the labels using the `randomChange` function.

The ROC curves and Confusion Matrices are automatically saved to the disk

```
import numpy as np
import pandas as pd
import matplotlib.pyplot as plt
import seaborn as sns
import json
from sklearn.preprocessing import MinMaxScaler
from sklearn.model_selection import cross_val_score
from sklearn.svm import SVC
from sklearn.metrics import roc_auc_score, roc_curve
from sklearn.metrics import confusion_matrix

drop_features = ['pkSeqID', 'proto',
                 'saddr', 'sport', 'daddr', 'dport',
                 'attack', 'category', 'subcategory']

y_feature = 'attack'

flipAmount = {0.00: "zero", 0.05: "five", 0.10: "ten",
              0.15: "fifteen", 0.20: "twenty", 0.25: "twentyfive",
              0.30: "thirty", 0.35: "thirtyfive", 0.40: "fourty",
              0.45: "fourtyfive", 0.50: "fifty"}

non_target_result = {'accuracy': [],
                     'precision': [],
                     'recall': [],
                     'f1_score': []}

for flip, name in flipAmount.items():
    print(f"[info] Starting now\n")
    index = name

    # Flip data
    flipdata = pd.read_csv('data/TrainTestSet/tenbest/tenbest-train-test-
split/UNSW_2018_IoT_Botnet_Final_10_best_Training.csv',
                           low_memory=False) # Load dataset
    change = randomChange(flip)
    flipdata.loc[change, 'attack'] ^= 1 # change by xor

    X_train = flipdata.drop(drop_features, axis=1)
    X_test = testing.drop(drop_features, axis=1)

    X_train_scaled = MMScaler(X_train)
    X_test_scaled = MMScaler(X_test)

    fullX = pd.concat([X_train_scaled, X_test_scaled])
    fullX_scaled = MMScaler(fullX)
```

```
    y_train = flipdata[y_feature]
    y_test = testing[y_feature]
    fullY = pd.concat([y_train, y_test])

    hyperparams = {'C':1,
                   'class_weight':'balanced',
                   'kernel':'linear',
                   'max_iter':1000}

    svcModel = SVC(**hyperparams)
    svcModel.fit(X_train_scaled, y_train)

    print(f"[+] Done! Scoring model: \n")

    y_proba = model.decision_function(X_test_scaled)
    auc = roc_auc_score(y_test, y_proba)
    fpr, tpr, thresholds = roc_curve(y_test, y_proba)
    plot_roc_curve(fpr, tpr, auc, flip=str(flip), targeted='False')

    accuracy = np.mean(cross_val_score(model, fullX_scaled, fullY, cv=4,
scoring='accuracy', n_jobs=-1))
    recall = np.mean(cross_val_score(model, fullX_scaled, fullY, cv=4,
scoring='recall', n_jobs=-1))
    precision = np.mean(cross_val_score(model, fullX_scaled, fullY, cv=4,
scoring='precision', n_jobs=-1))
    f1_score = np.mean(cross_val_score(model, fullX_scaled, fullY, cv=4,
scoring='f1', n_jobs=-1))

    for key, value in non_target_result.items():
        if key == 'accuracy':
            non_target_result[key].append(accuracy)
        if key == 'recall':
            non_target_result[key].append(recall)
        if key == 'precision':
            non_target_result[key].append(precision)
        if key == 'f1_score':
            non_target_result[key].append(f1_score)

    y_pred = model.predict(X_test_scaled)
    conf_mat = confusion_matrix(y_test, y_pred)
    labels = ['Benign', 'Attack']
    plot_conf_mat(conf_mat, labels=labels, flip=str(flip),
targeted='False') # run cell above for accurate result

    print(f"[info] Cleaning up")
    del model
    del change
    del flipdata
    del X_train, X_train_scaled, fullX, fullX_scaled
    del y_train, y_test, fullY

with open("models/non_targeted_svm_result.json", 'w') as file:
    json.dump(non_targeted_result, file)
```

## Targeted SVC label flipping

Here we flip the labels using the `targetChange` function.

The ROC curves and Confusion Matrices are automatically saved to the disk

```
import numpy as np
import pandas as pd
import matplotlib.pyplot as plt
import seaborn as sns
import json, pickle
from sklearn.preprocessing import MinMaxScaler
from sklearn.model_selection import cross_val_score
from sklearn.svm import SVC
from sklearn.metrics import roc_auc_score, roc_curve
from sklearn.metrics import confusion_matrix

drop_features = ['pkSeqID', 'proto',
                 'saddr', 'sport', 'daddr', 'dport',
                 'attack', 'category', 'subcategory']

y_feature = 'attack'

flipAmount = {0.00: "zero", 0.05: "five", 0.10: "ten",
              0.15: "fifteen", 0.20: "twenty", 0.25: "twentyfive",
              0.30: "thirty", 0.35: "thirtyfive", 0.40: "fourty",
              0.45: "fourtyfive", 0.50: "fifty"}

target_result = {'accuracy': [],
                 'precision': [],
                 'recall': [],
                 'f1_score': []}

defaultModel = pickle.load(open("models/SVM/trusted_model.pk1", "rb"))

for flip, name in flipAmount.items():
    print(f"[info] Starting now\n")
    index = name

    # Flip data
    flipdata = pd.read_csv('data/TrainTestSet/tenbest/tenbest-train-test-
split/UNSW_2018_IoT_Botnet_Final_10_best_Training.csv',
                          low_memory=False) # Load dataset
    # Get index to flip labels
    default_X_train = training.drop(drop_features, axis=1)
    default_X_train_scaled = MMScaler(default_X_train)

    change = targetChange(defaultModel, default_X_train_scaled, flip)
    flipdata.loc[change, 'attack'] ^= 1 # change by xor

    X_train = flipdata.drop(drop_features, axis=1)
    X_test = testing.drop(drop_features, axis=1)
```

```
    X_train_scaled = MMScaler(X_train)
    X_test_scaled = MMScaler(X_test)

    fullX = pd.concat([X_train_scaled, X_test_scaled])
    fullX_scaled = MMScaler(fullX)

    y_train = flipdata[y_feature]
    y_test = testing[y_feature]
    fullY = pd.concat([y_train, y_test])

    hyperparams = {'C':1,
                   'class_weight':'balanced',
                   'kernel':'linear',
                   'max_iter':1000}

    svcModel = SVC(**hyperparams)
    svcModel.fit(X_train_scaled, y_train)

    print(f"[+] Done! Scoring model: \n")

    y_proba = model.decision_function(X_test_scaled)
    auc = roc_auc_score(y_test, y_proba)
    fpr, tpr, thresholds = roc_curve(y_test, y_proba)
    plot_roc_curve(fpr, tpr, auc, flip=str(flip), targeted='True')

    accuracy = np.mean(cross_val_score(model, fullX_scaled, fullY, cv=4,
scoring='accuracy', n_jobs=-1))
    recall = np.mean(cross_val_score(model, fullX_scaled, fullY, cv=4,
scoring='recall', n_jobs=-1))
    precision = np.mean(cross_val_score(model, fullX_scaled, fullY, cv=4,
scoring='precision', n_jobs=-1))
    f1_score = np.mean(cross_val_score(model, fullX_scaled, fullY, cv=4,
scoring='f1', n_jobs=-1))

    for key, value in target_result.items():
        if key == 'accuracy':
            target_result[key].append(accuracy)
        if key == 'recall':
            target_result[key].append(recall)
        if key == 'precision':
            target_result[key].append(precision)
        if key == 'f1_score':
            target_result[key].append(f1_score)

    y_pred = model.predict(X_test_scaled)
    conf_mat = confusion_matrix(y_test, y_pred)
    labels = ['Benign', 'Attack']
    plot_conf_mat(conf_mat, labels=labels, flip=str(flip), targeted='True')
# run cell above for accurate result

    print(f"[info] Cleaning up")
    del model
    del change
```

```
    del flipdata
    del X_train, X_train_scaled, fullX, fullX_scaled
    del y_train, y_test, fullY

with open("models/targeted_svm_result.json", 'w') as file:
    json.dump(targeted_result, file)
```

## 6. Plot line graphs

```
with open("models/non_targeted_svm_result.json", "r") as file:
    non_targeted_svm_result = json.load(file)

with open("models/targeted_svm_result.json", "r") as file:
    targeted_svm_result = json.load(file)
```

Random label flip

```
import matplotlib.pyplot as plt
Xscale = [0.0, 5, 10, 15, 20, 25, 30, 35, 40, 45, 50]

fig, ax = plt.subplots(2, 2, figsize=(8, 5))

ax[0, 0].plot(Xscale, non_targeted_svm_result['accuracy'], 'tab:red')
ax[0, 0].set_title('Accuracy Score')
ax[0, 0].set_ylim([0, 1.1])
ax[0, 1].plot(Xscale, non_targeted_svm_result['recall'])
ax[0, 1].set_title('Recall Score')
ax[0, 1].set_ylim([0, 1.1])
ax[1, 0].plot(Xscale, non_targeted_svm_result['precision'], 'tab:orange')
ax[1, 0].set_title('Precision Score')
ax[1, 0].set_ylim([0, 1.1])
ax[1, 1].plot(Xscale, non_targeted_svm_result['f1_score'], 'tab:purple')
ax[1, 1].set_title('F1 Score')
ax[1, 1].set_ylim([0, 1.1])

for a in ax.flat:
    a.set(xlabel='Label Flip Percentage')
fig.tight_layout(pad=2)
```

Targeted label flip

```
import matplotlib.pyplot as plt
Xscale = [0.0, 5, 10, 15, 20, 25, 30, 35, 40, 45, 50]

fig, ax = plt.subplots(2, 2, figsize=(8, 5))
```

```
ax[0, 0].plot(Xscale, targeted_svm_result['accuracy'], 'tab:red')
ax[0, 0].set_title('Accuracy Score')
ax[0, 0].set_ylim([0.4, 1.1])
ax[0, 1].plot(Xscale, targeted_svm_result['recall'])
ax[0, 1].set_title('Recall Score')
ax[0, 1].set_ylim([0.4, 1.1])
ax[1, 0].plot(Xscale, targeted_svm_result['precision'], 'tab:orange')
ax[1, 0].set_title('Precision Score')
ax[1, 0].set_ylim([0.4, 1.1])
ax[1, 1].plot(Xscale, targeted_svm_result['f1_score'], 'tab:purple')
ax[1, 1].set_title('F1 Score')
ax[1, 1].set_ylim([0.4, 1.1])

for a in ax.flat:
    a.set(xlabel='Label Flip Percentage')
fig.tight_layout(pad=2)
```

Zoom in on the recall score

```
import matplotlib.pyplot as plt

svm_recall_only = {'targeted': targeted_svm_result['recall'],
                   'non_targeted': non_targeted_svm_result['recall']}

Xscale = [0.0, 5, 10, 15, 20, 25, 30, 35, 40, 45, 50]

fig, ax = plt.subplots(1, 1, figsize=(7, 5))

ax.plot(Xscale, svm_recall_only['targeted'], label='Targeted')
ax.plot(Xscale, svm_recall_only['non_targeted'], '--', label='Not Targeted
Recall')
ax.set_title('Comparing recall score in targeted / non-targeted SVM label
flip')
ax.set_ylim([0.55, 1.05])

ax.set_xlabel('Label Flip (Percentage)')
ax.set_ylabel('Recall Score')
ax.legend()
leg = ax.legend();
```
