# Supplementary material for: Launching Adversarial Attacks against Network Intrusion Detection Systems for IoT
Source: arXiv:2104.12426 source file (2021-04-26)
Supplement: Supplementary file 6 [file Appendix_B.tex]

\chapter{Project Management}
\label{app:proj_mgmt}

\includepdf[pages=1, width=\textwidth, frame, pagecommand=\section{Gantt Chart}, offset=0 -1.3cm]{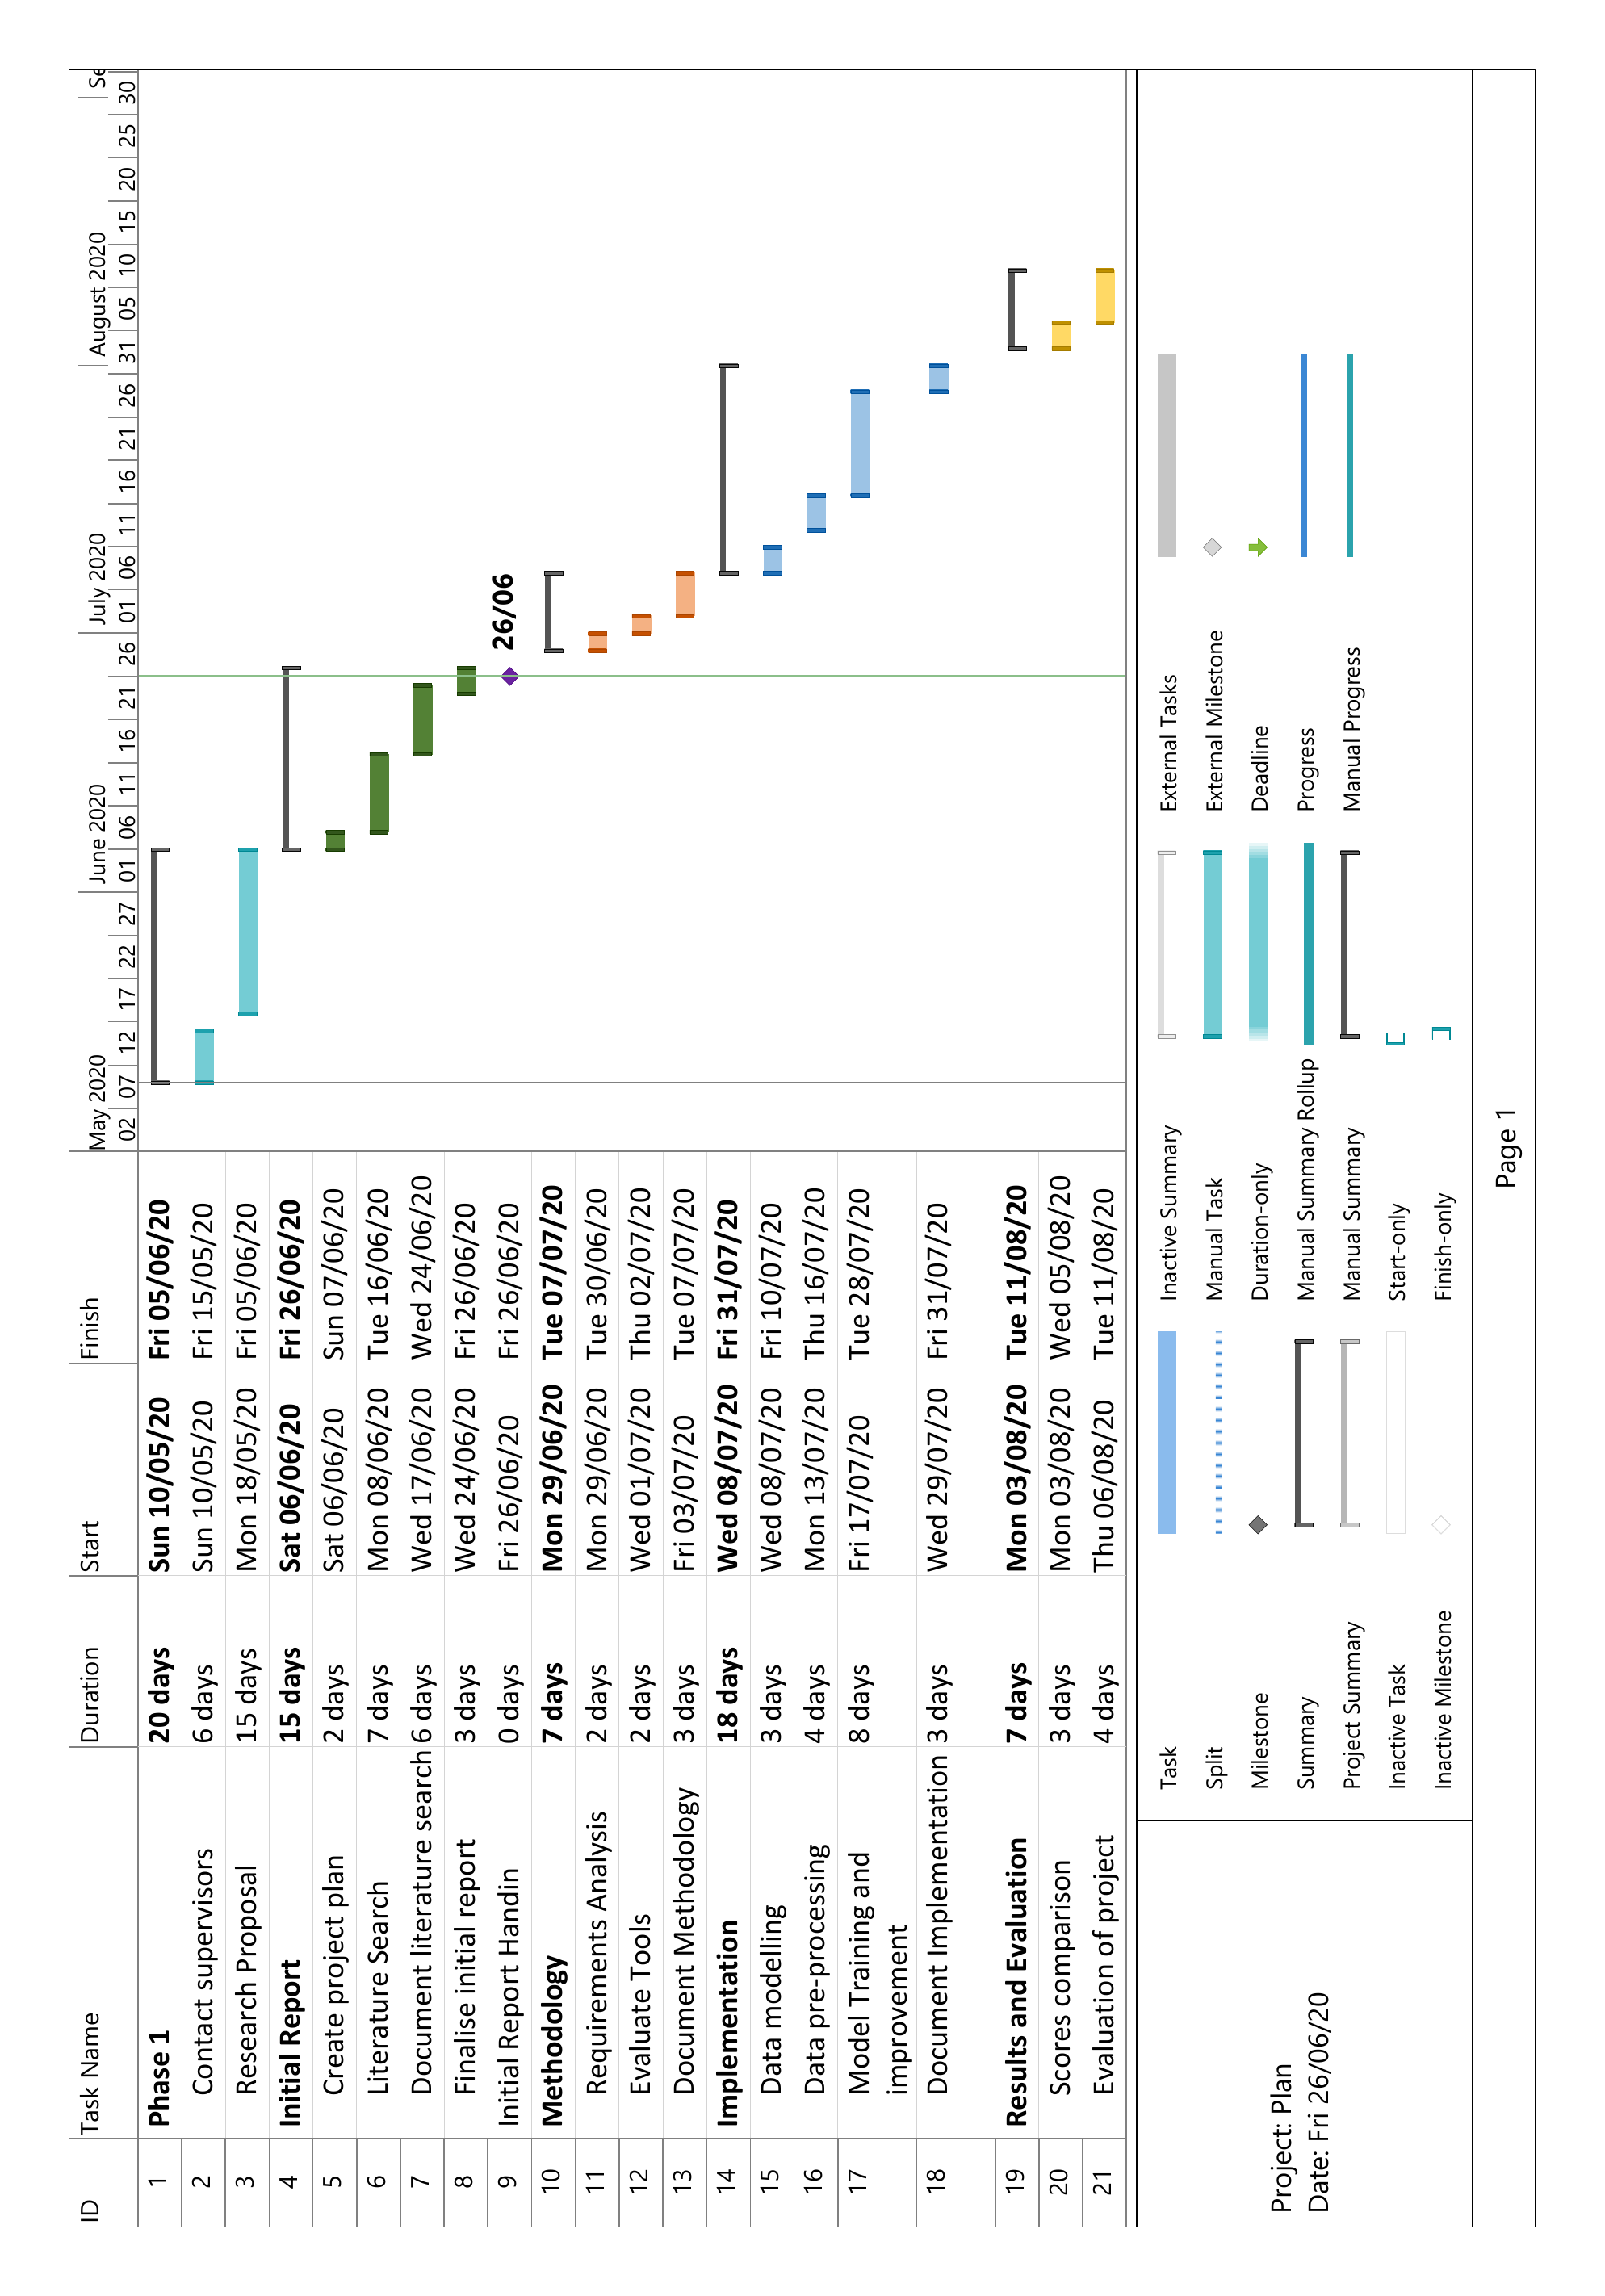}
\includepdf[pages=2-, width=\textwidth, frame, pagecommand={}, offset=0 -1.3cm]{./appendices/ganttChart.pdf}

% June 26 [Initial Report]
\includepdf[pages=1, width=\textwidth, frame, pagecommand=\section{Initial Report}, offset=0 -1.3cm]{./diaries/initial_report.pdf}
\includepdf[pages=2-, width=\textwidth, frame, pagecommand={}, offset=0 -1.3cm]{./diaries/initial_report.pdf}

% July 7 [Initial Report Feedback]
\includepdf[pages=1, width=\textwidth, frame, pagecommand=\section{Initial Report Feedback}, offset=0 -1.3cm]{./diaries/initial_report_feedback.pdf}
