# Supplementary material for: Launching Adversarial Attacks against Network Intrusion Detection Systems for IoT
Source: arXiv:2104.12426 source file (2021-04-26)
Supplement: Supplementary file 7 [file Appendix_D.tex]

\chapter{Jupyter Notebooks}
\label{app:jupyter}

\includepdf[pages=1, width=\textwidth, frame, pagecommand=\section{SVM Model Manipulation}, offset=0 -1.3cm]{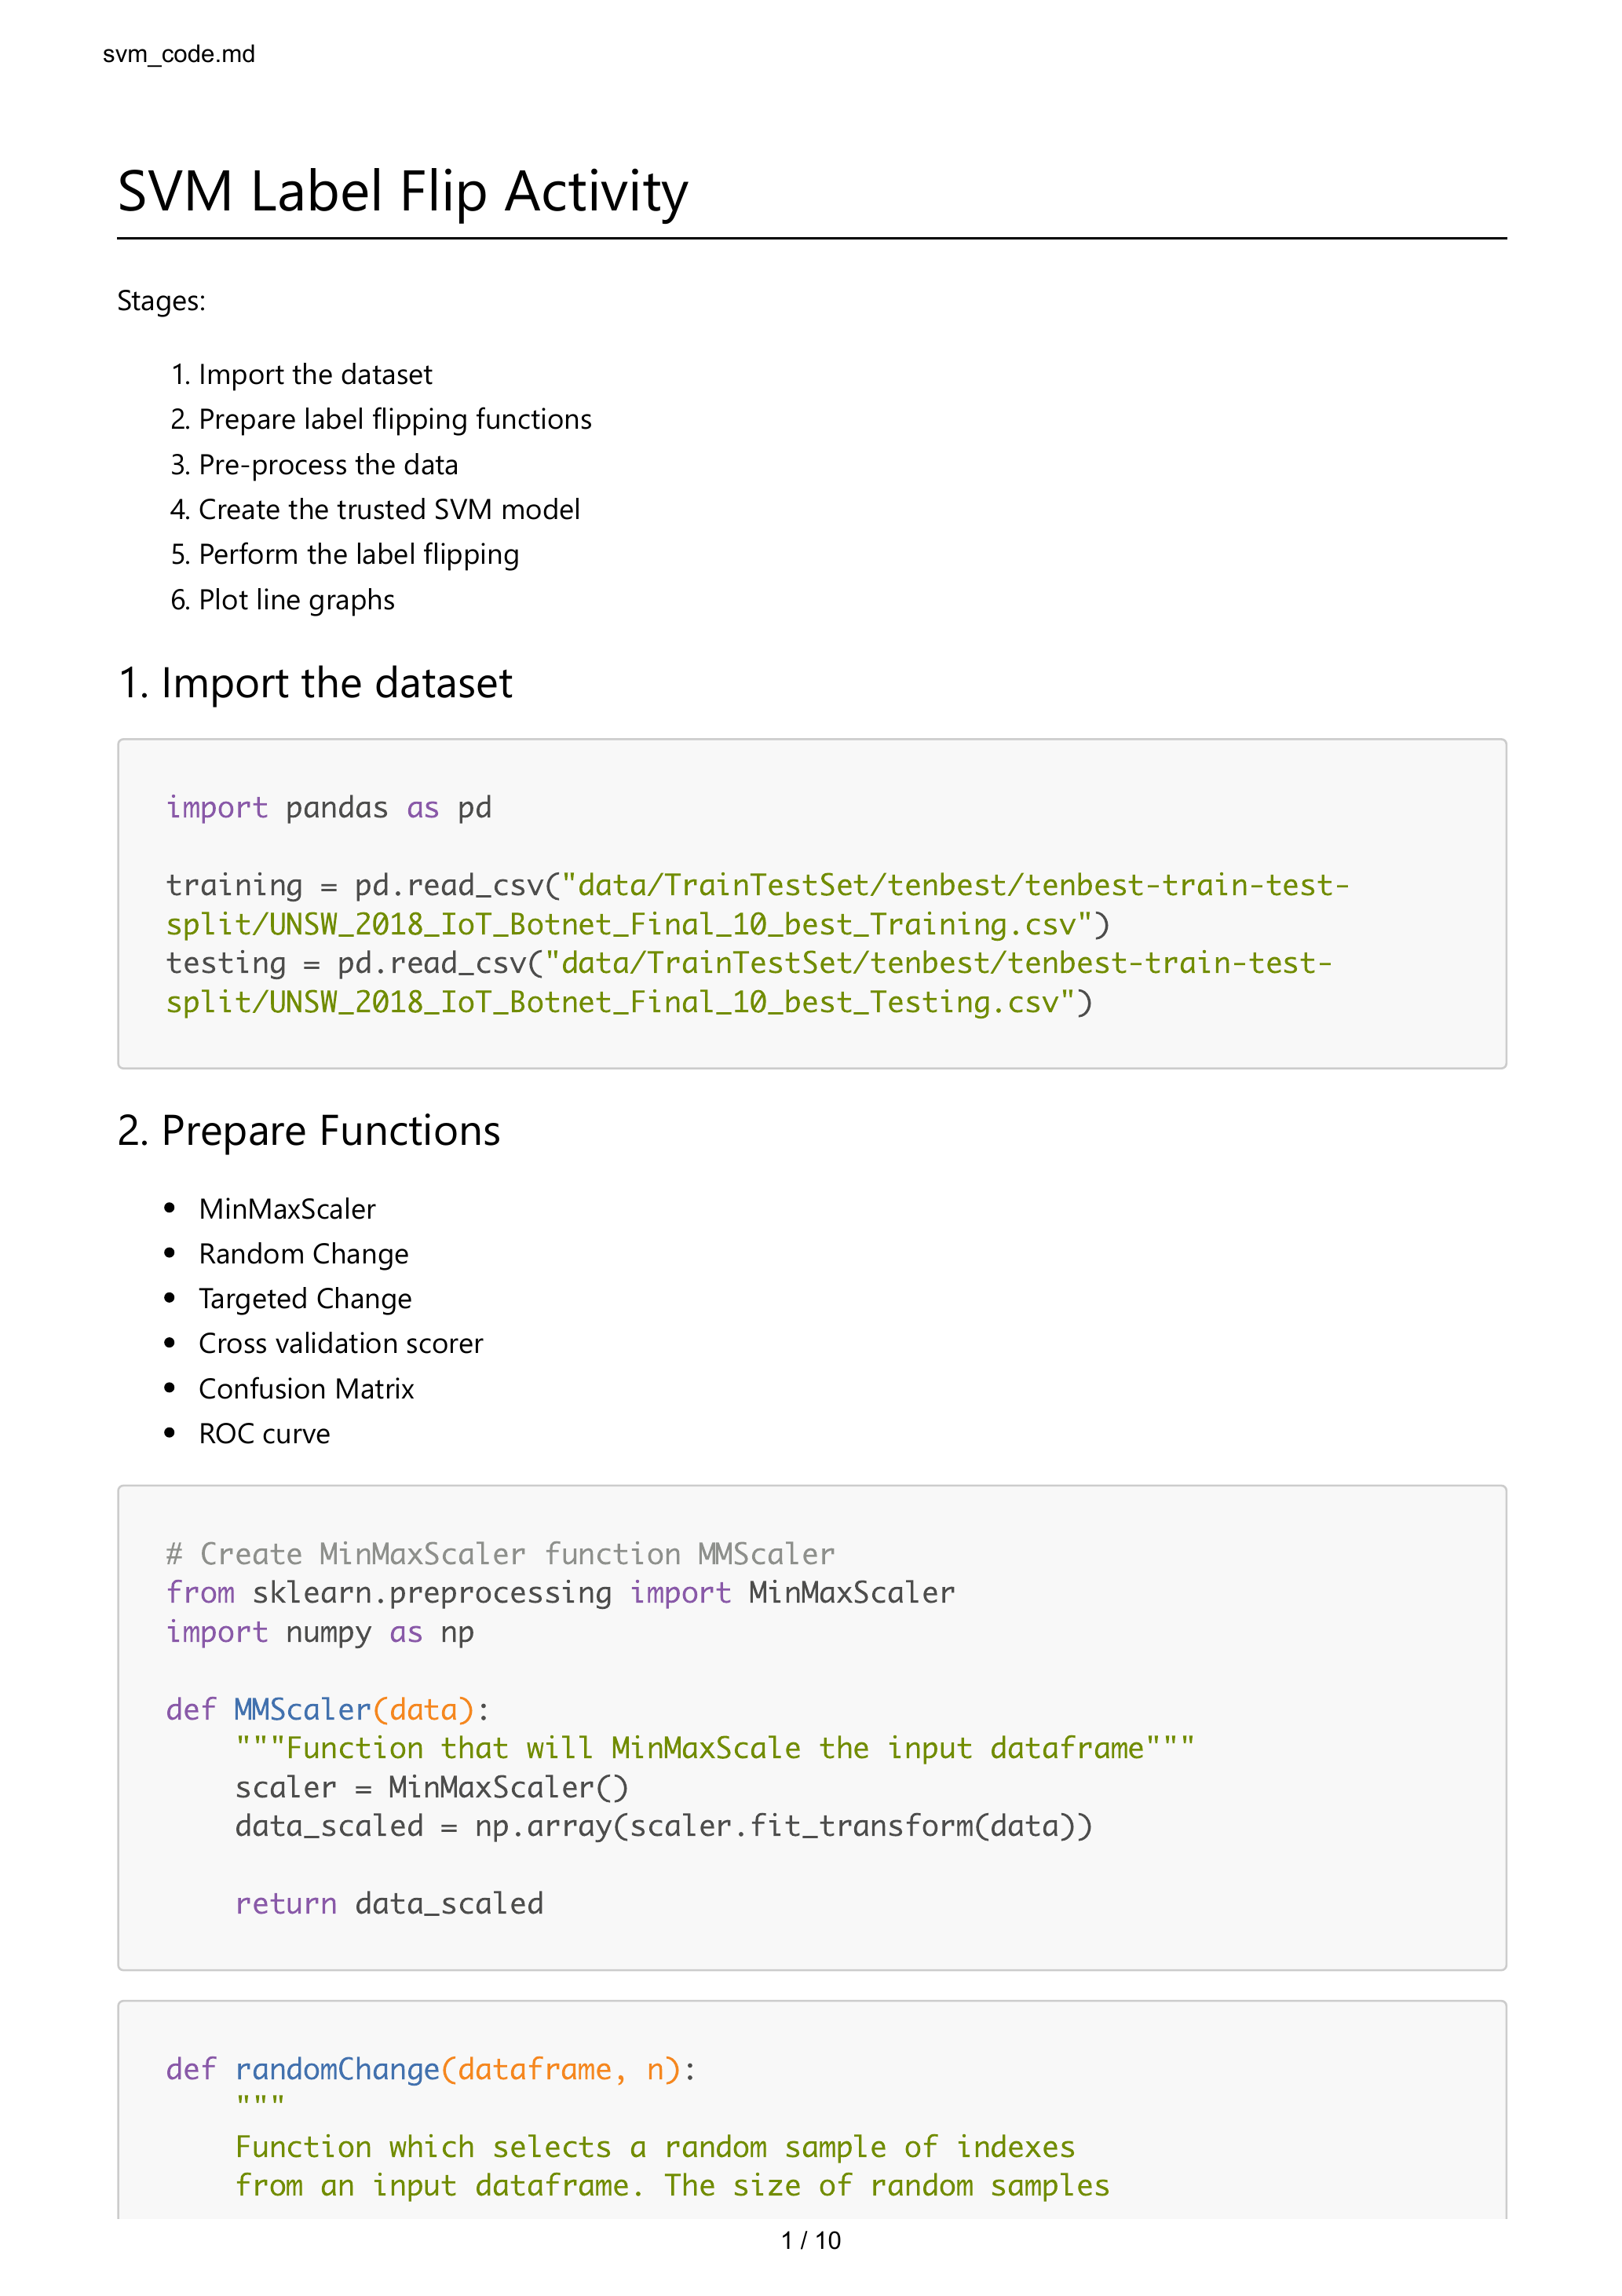}
\includepdf[pages=2-, width=\textwidth, frame, pagecommand={}, offset=0 -1.3cm]{./appendices/svm_code.pdf}

\includepdf[pages=1, width=\textwidth, frame, pagecommand=\section{ANN Model Evasion}, offset=0 -1.3cm]{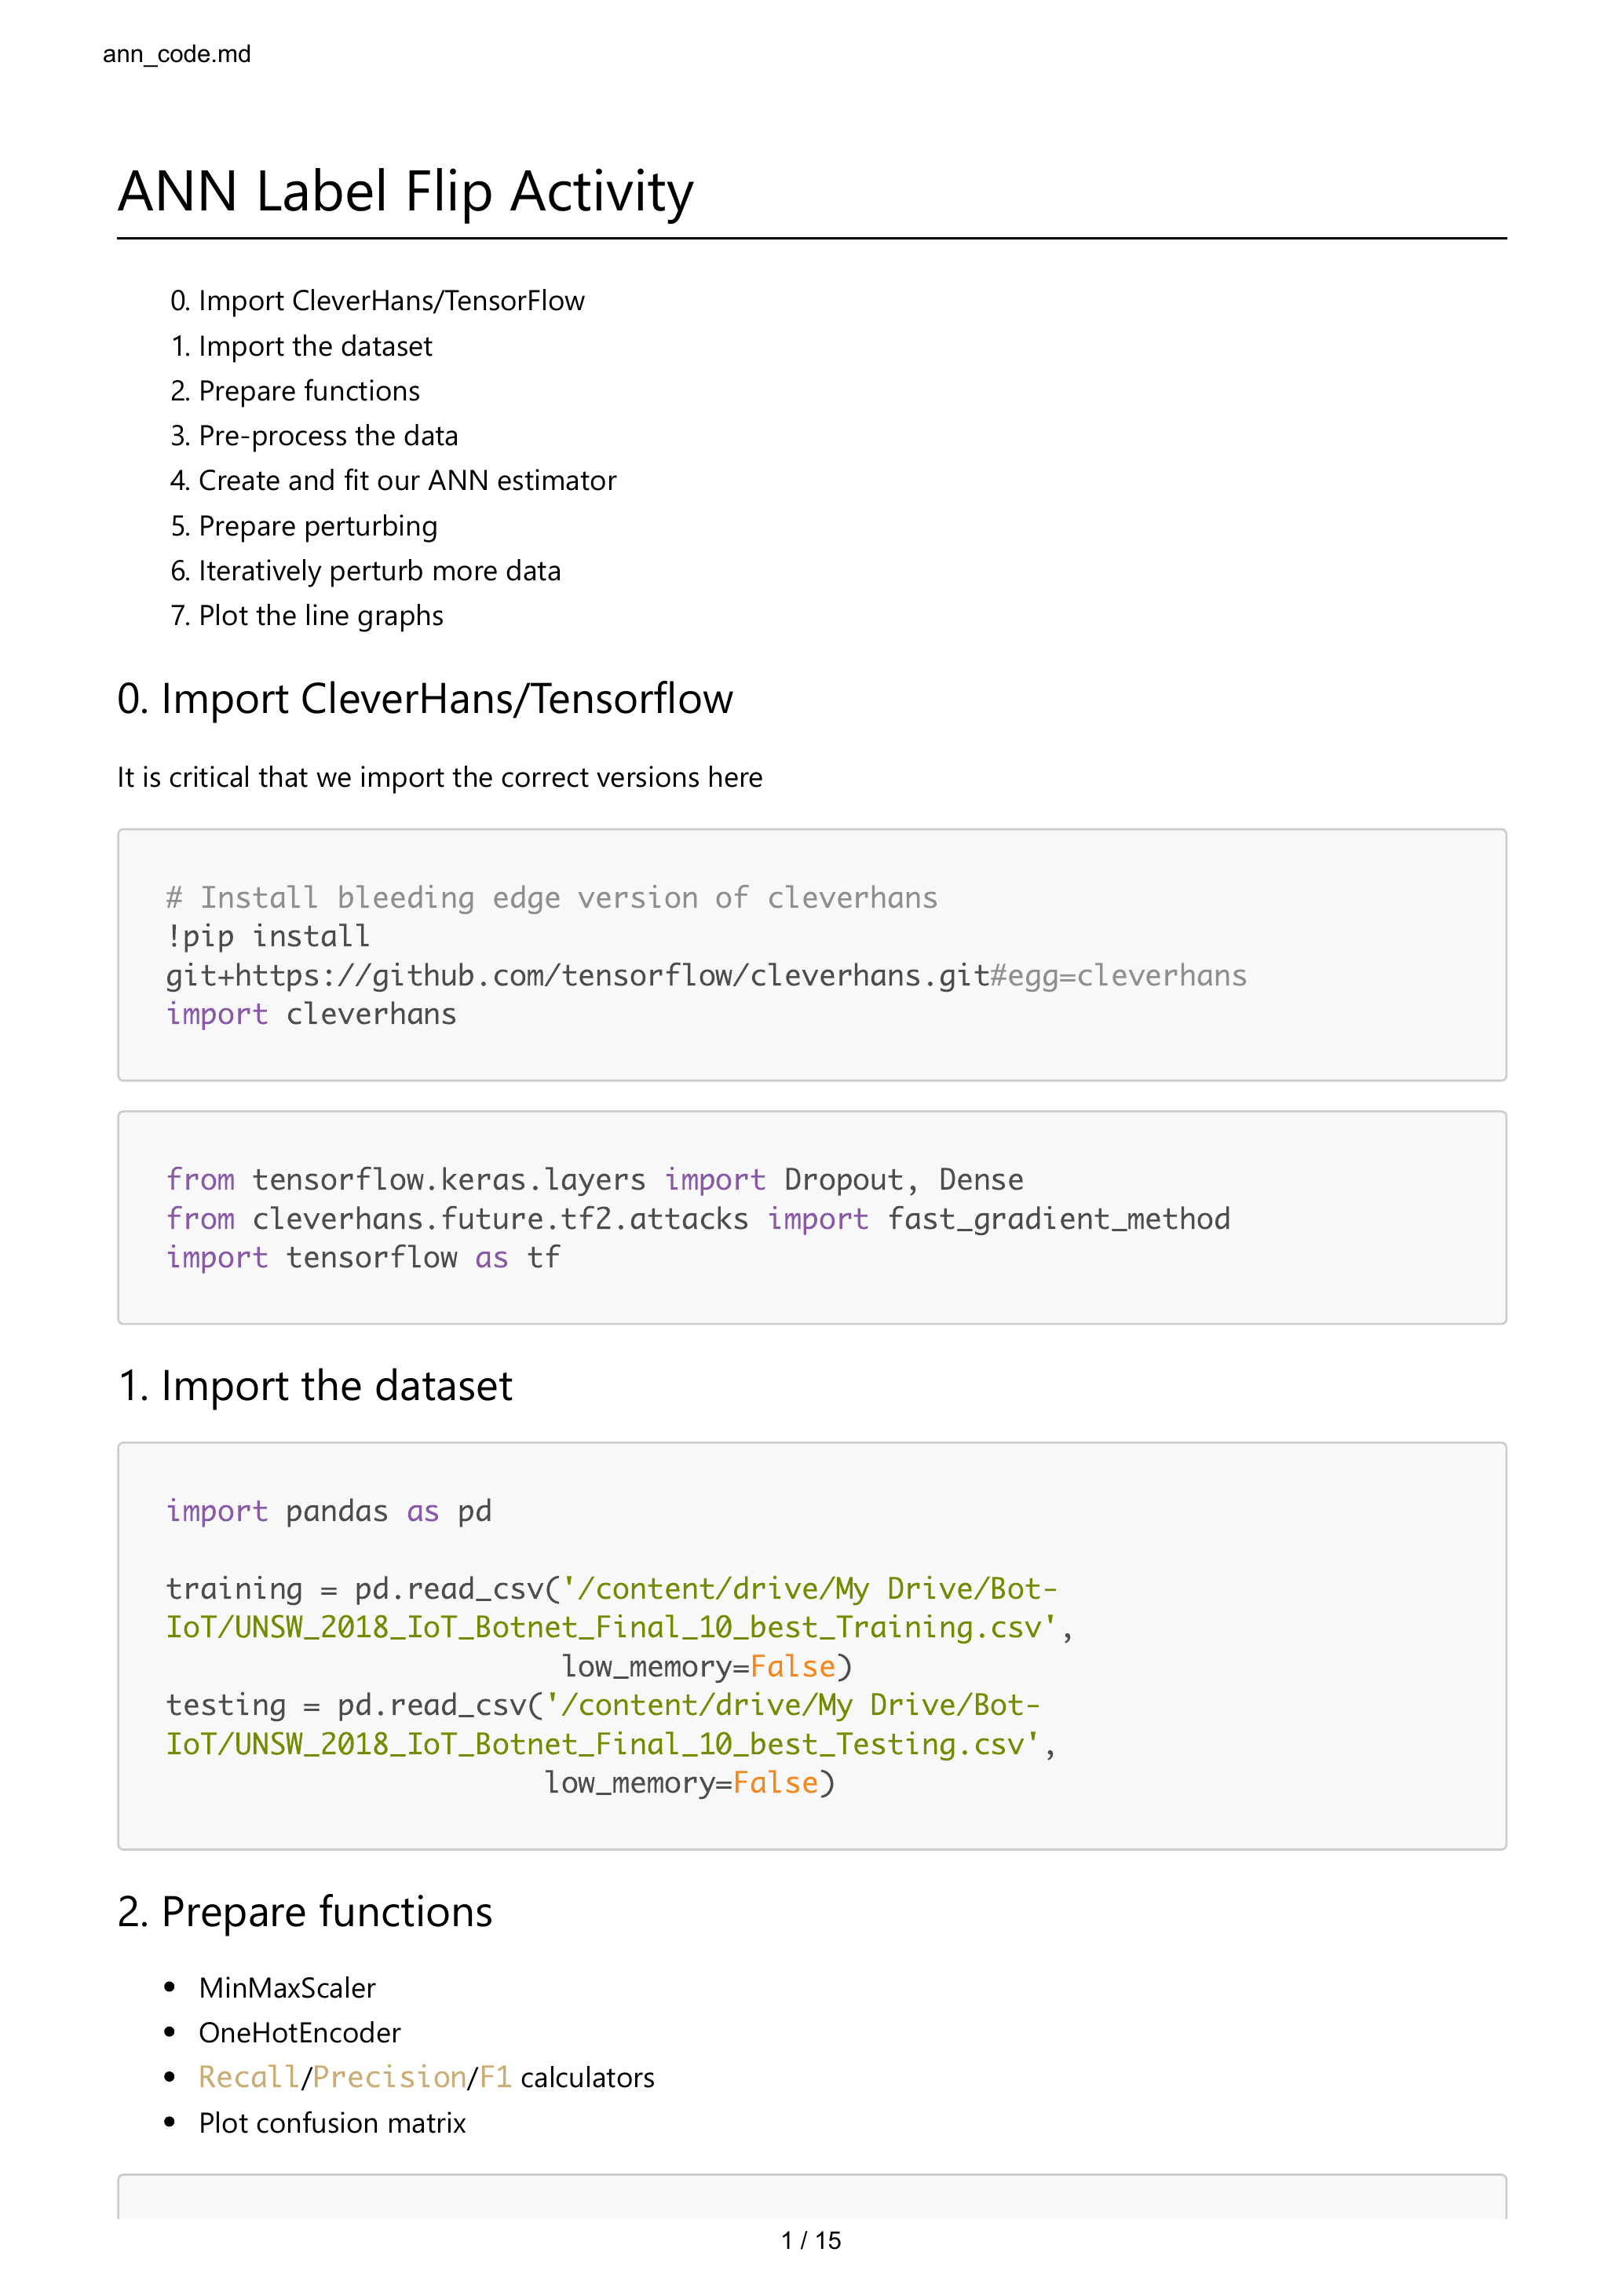}
\includepdf[pages=2-, width=\textwidth, frame, pagecommand={}, offset=0 -1.3cm]{./appendices/ann_code.pdf}
