# Supplementary material for: Launching Adversarial Attacks against Network Intrusion Detection Systems for IoT
Source: arXiv:2104.12426 source file (2021-04-26)
Supplement: Supplementary file 8 [file appendix_A.tex]

\chapter{Project Initiation}
\label{app:proj_proposal}

\includepdf[pages=1, width=\textwidth, frame, pagecommand=\section{Project Proposal}, offset=0 -1.3cm]{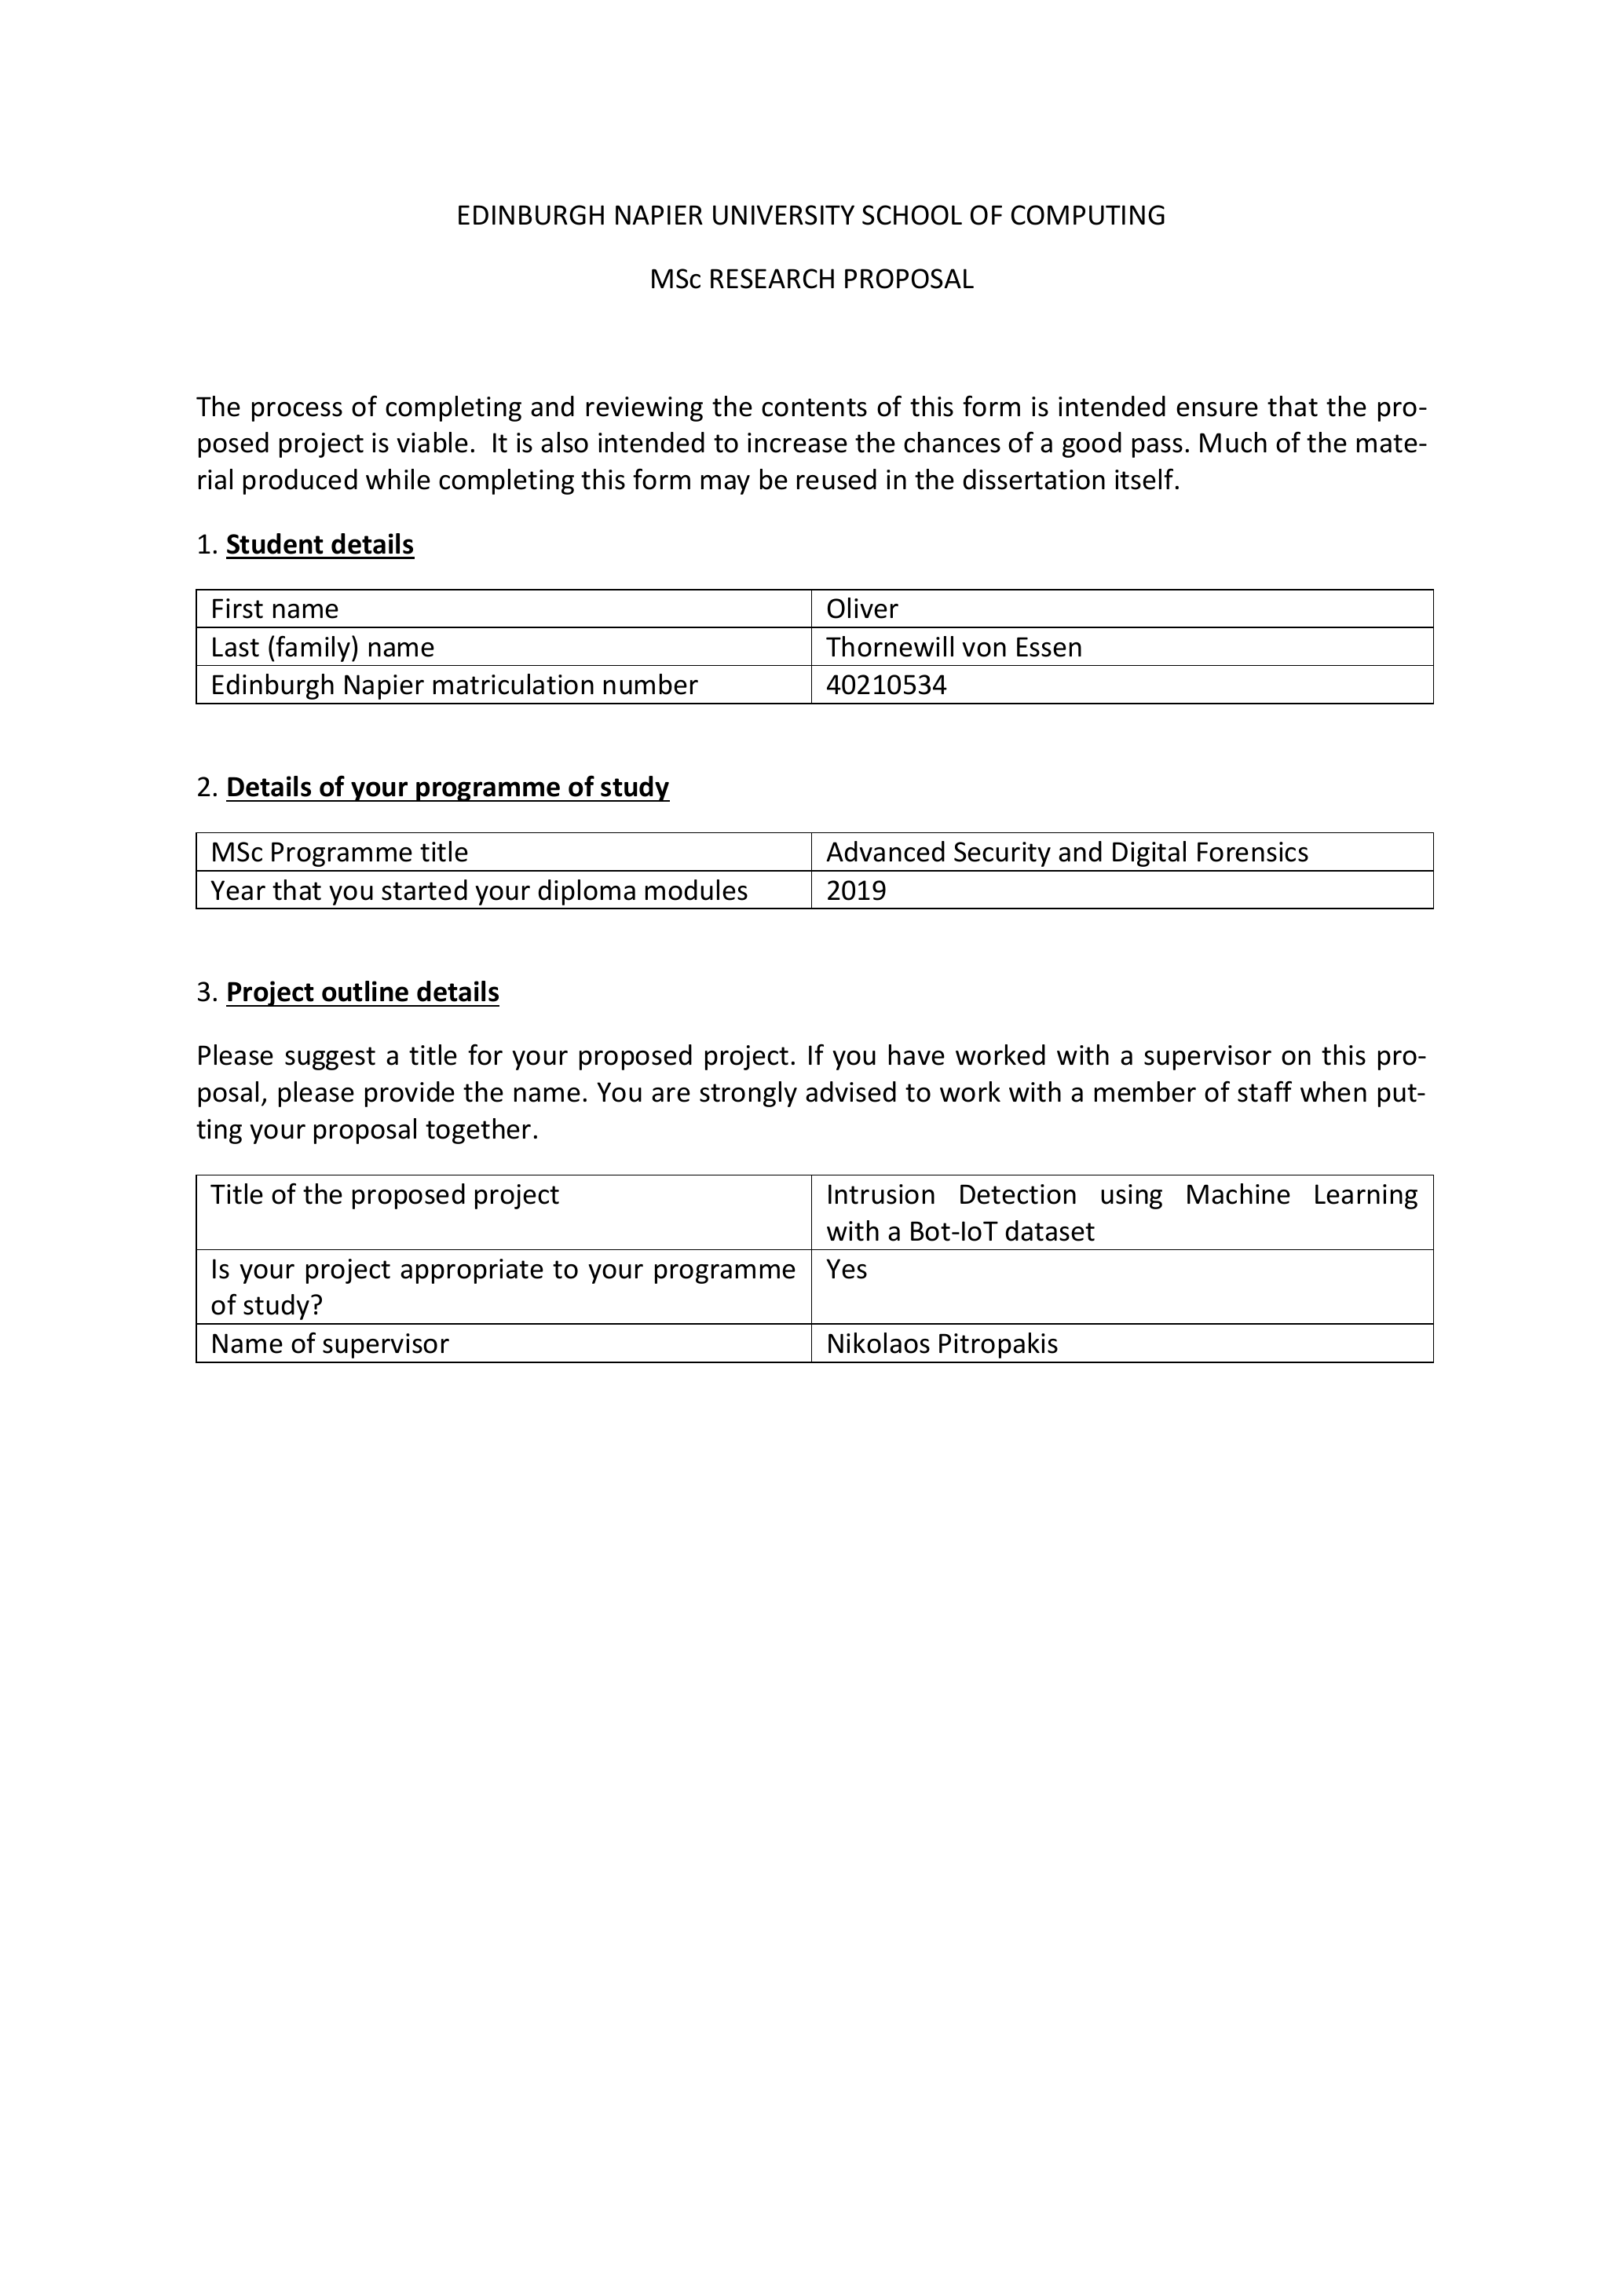}
\includepdf[pages=2-, width=\textwidth, frame, pagecommand={}, offset=0 -1.3cm]{./appendices/proj_proposal.pdf}

\includepdf[pages=1, width=\textwidth, frame, pagecommand=\section{Project Propsal Feedback}, offset=0 -1.3cm]{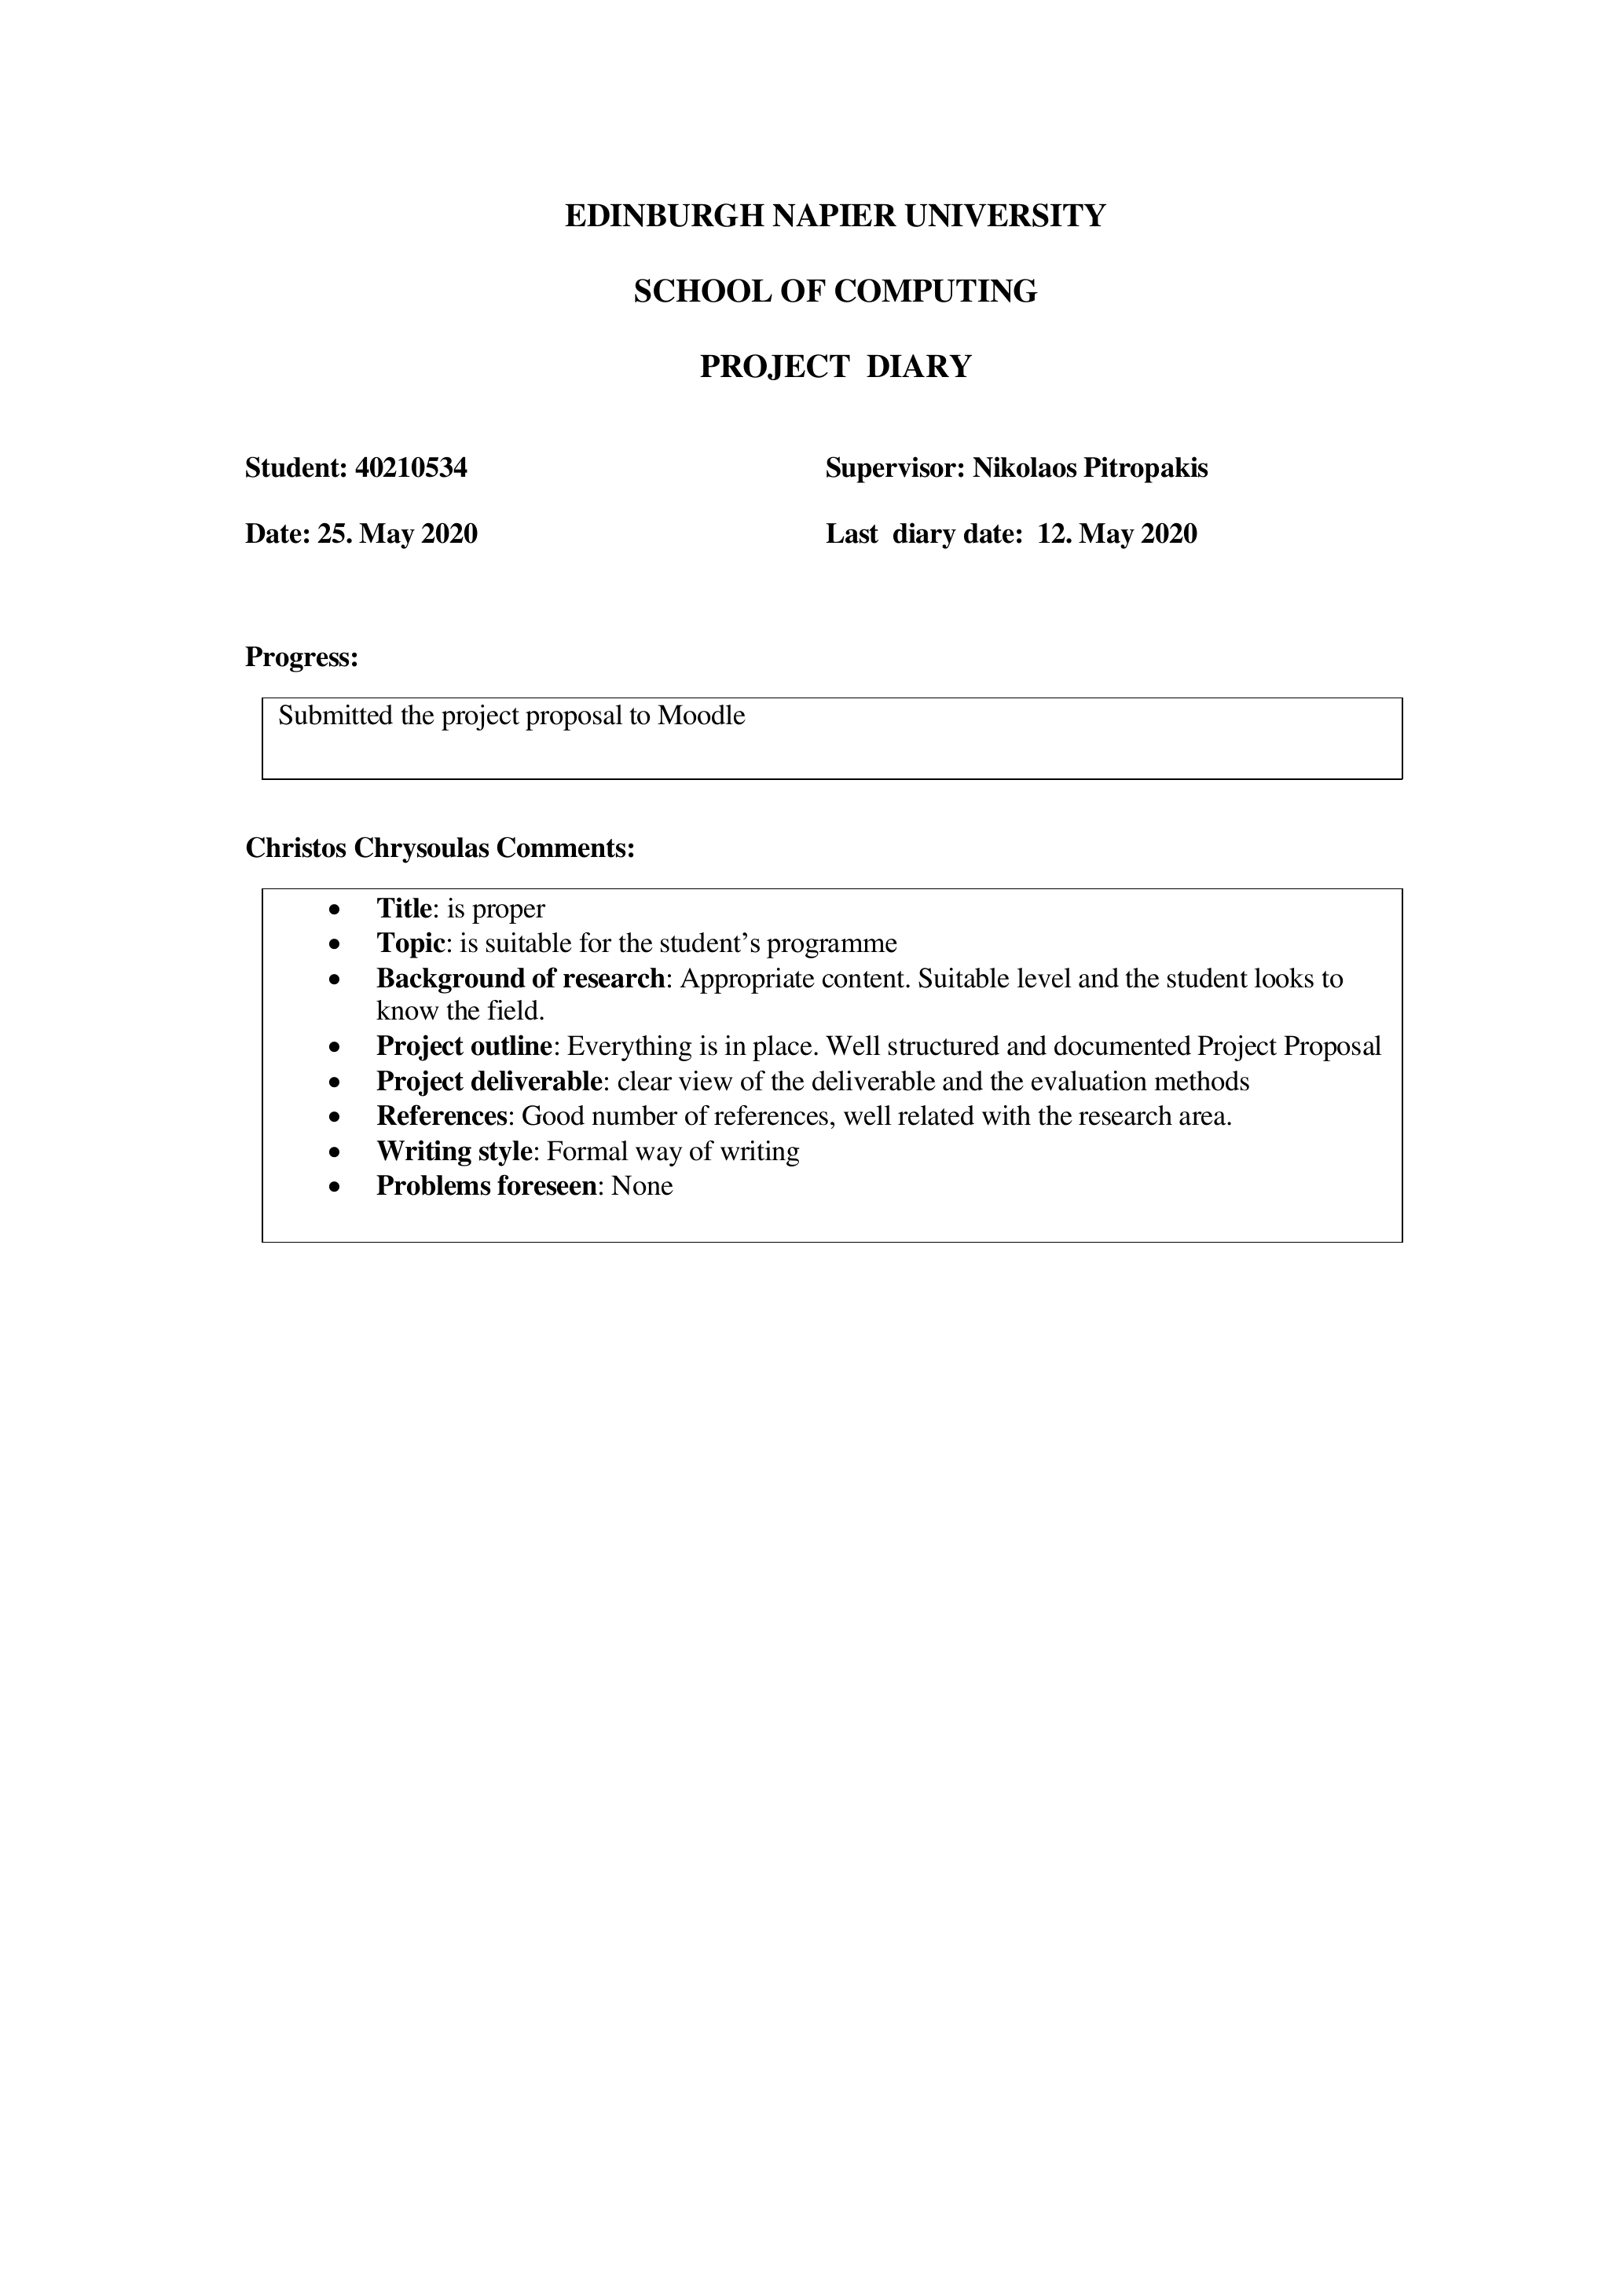}
